# Supplementary material for: Massive Star Population in the Sextans A Dwarf Galaxy from HST UV Photometry
Source: arXiv:2602.07177 ancillary file (2026-02-06)
Supplement: Supplementary file 1 [file Catalog.pdf]

Table 1: Key to Table 2.

| Column                                                         | Value                                                  |
|----------------------------------------------------------------|--------------------------------------------------------|
| <b>IDN</b>                                                     | Unique serial identifier                               |
| <b>Zone</b>                                                    | Region of the CMD (ZAMS L/MS/TAMS R)                   |
| <b>M</b>                                                       | ZAMS mass ( $M_{\odot}$ )                              |
| <b><math>\sigma_M</math></b>                                   | Uncertainty of M                                       |
| <b>RA, Dec</b>                                                 | Right ascension/declination in ICRS (degree)           |
| <b>F275, F336</b>                                              | Apparent magnitude in F275W/F336W filter (Vega system) |
| <b><math>\sigma_{F275}, \sigma_{F336}</math></b>               | Uncertainty of F275/F336                               |
| <b>x, y</b>                                                    | Coordinates in CMD (mag)                               |
| <b><math>d_x/\sigma_x</math></b>                               | Distance to MS tracks in standard deviations of color  |
| <b>Age</b>                                                     | Stellar age (Ma)                                       |
| <b>log(T)</b>                                                  | Decimal logarithm of effective temperature (K)         |
| <b>log(g)</b>                                                  | Decimal logarithm of surface gravity (Gal)             |
| <b><math>\sigma_{Age}, \sigma_{logT}, \sigma_{logg}</math></b> | Uncertainty of Age/log(T)/log(g)                       |

Table 2 - Catalog of massive main sequence stars in Sextans A. See key in Table 1.

| IDN | Zone   | M    | $\sigma_M$ | RA          | Dec        | F275   | F336   | $\sigma_{F275}$ | $\sigma_{F336}$ | x      | y      | $d_x/\sigma_x$ | Age  | log(T) | log(g) | $\sigma_{Age}$ | $\sigma_{logT}$ | $\sigma_{logg}$ |
|-----|--------|------|------------|-------------|------------|--------|--------|-----------------|-----------------|--------|--------|----------------|------|--------|--------|----------------|-----------------|-----------------|
| 1   | ZAMS L | 57.9 | 10.9       | 152.7241585 | -4.6869743 | 18.277 | 18.91  | 0.021           | 0.018           | -0.706 | -7.737 | 0.87           | 0    | 4.73   | 4.37   | 2.4            | 0.1             | 0.33            |
| 2   | MS     | 50.4 | 20.8       | 152.7411774 | -4.7195234 | 18.441 | 19.06  | 0.028           | 0.025           | -0.692 | -7.573 | 0.02           | 0.6  | 4.7    | 4.31   | 3.9            | 0.1             | 0.36            |
| 3   | MS     | 38.2 | 6          | 152.7266164 | -4.6867412 | 18.971 | 19.581 | 0.021           | 0.019           | -0.683 | -7.043 | -              | 0.1  | 4.67   | 4.37   | 0.2            | 0.05            | 0.13            |
| 4   | MS     | 36.4 | 10.6       | 152.7420465 | -4.695847  | 19.069 | 19.678 | 0.039           | 0.028           | -0.682 | -6.945 | -              | 0    | 4.67   | 4.39   | 0.5            | 0.1             | 0.24            |
| 5   | MS     | 35.5 | 13         | 152.7344452 | -4.7147598 | 18.347 | 18.947 | 0.022           | 0.026           | -0.673 | -7.667 | -              | 4.2  | 4.64   | 4.04   | 3.3            | 0.1             | 0.36            |
| 6   | MS     | 34.6 | 12         | 152.7246869 | -4.6924857 | 18.846 | 19.45  | 0.016           | 0.018           | -0.677 | -7.168 | -              | 2.1  | 4.66   | 4.26   | 4.2            | 0.06            | 0.23            |
| 7   | MS     | 34.4 | 13.9       | 152.7289993 | -4.6878345 | 19.042 | 19.646 | 0.028           | 0.019           | -0.677 | -6.972 | -              | 0.7  | 4.66   | 4.33   | 5.6            | 0.11            | 0.39            |
| 8   | ZAMS   | 31.8 | 7          | 152.7247133 | -4.6826297 | 19.293 | 19.927 | 0.018           | 0.02            | -0.707 | -6.721 | 1.53           | 0    | 4.66   | 4.4    | 0.6            | 0.08            | 0.2             |
| 9   | ZAMS L | 30.4 | 7.6        | 152.7685622 | -4.7016954 | 19.362 | 19.975 | 0.022           | 0.021           | -0.686 | -6.652 | 0.51           | 0    | 4.65   | 4.4    | 0.6            | 0.09            | 0.22            |
| 10  | TAMS R | 30.4 | 3.5        | 152.738782  | -4.6820961 | 17.725 | 18.279 | 0.018           | 0.025           | -0.627 | -8.289 | 1.47           | 6.9  | 4.55   | 3.57   | 0.8            | 0.03            | 0.11            |
| 11  | ZAMS L | 29.5 | 9.7        | 152.7231391 | -4.6987162 | 19.412 | 20.021 | 0.02            | 0.023           | -0.682 | -6.602 | 0.36           | 0    | 4.65   | 4.4    | 1              | 0.13            | 0.31            |
| 12  | MS     | 26.7 | 8.4        | 152.7236118 | -4.6965713 | 19.472 | 20.073 | 0.021           | 0.016           | -0.674 | -6.542 | 0.09           | 0.9  | 4.62   | 4.34   | 6.1            | 0.09            | 0.32            |
| 13  | MS     | 25.8 | 7.5        | 152.7541659 | -4.6839293 | 19.428 | 20.024 | 0.022           | 0.016           | -0.669 | -6.586 | -              | 1.7  | 4.62   | 4.31   | 5.4            | 0.08            | 0.3             |
| 14  | MS     | 25.7 | 3.7        | 152.7368548 | -4.67803   | 18.126 | 18.708 | 0.024           | 0.024           | -0.655 | -7.888 | -              | 7.5  | 4.52   | 3.58   | 1.3            | 0.07            | 0.24            |
| 15  | ZAMS L | 25.4 | 10         | 152.7245159 | -4.6886963 | 19.662 | 20.261 | 0.021           | 0.022           | -0.672 | -6.352 | 0.1            | 0    | 4.62   | 4.41   | 1.5            | 0.16            | 0.39            |
| 16  | ZAMS L | 25.1 | 8.7        | 152.7282353 | -4.6816023 | 19.683 | 20.288 | 0.019           | 0.016           | -0.678 | -6.331 | 0.44           | 0    | 4.62   | 4.41   | 1.3            | 0.14            | 0.33            |
| 17  | ZAMS L | 23.8 | 10         | 152.7375668 | -4.6752915 | 19.775 | 20.383 | 0.022           | 0.017           | -0.681 | -6.239 | 0.57           | 0    | 4.61   | 4.41   | 2              | 0.18            | 0.45            |
| 18  | MS     | 22.2 | 5.9        | 152.7328866 | -4.6790161 | 19.869 | 20.462 | 0.023           | 0.02            | -0.666 | -6.145 | -              | 0    | 4.6    | 4.39   | 7              | 0.07            | 0.28            |
| 19  | ZAMS L | 22.1 | 6.5        | 152.7487614 | -4.6698171 | 19.91  | 20.508 | 0.026           | 0.021           | -0.671 | -6.104 | 0.15           | 0    | 4.6    | 4.41   | 7.8            | 0.09            | 0.33            |
| 20  | MS     | 22   | 7.3        | 152.7294757 | -4.6812802 | 19.954 | 20.548 | 0.021           | 0.022           | -0.667 | -6.06  | -              | -0.1 | 4.61   | 4.44   | 8.5            | 0.1             | 0.38            |

| IDN | Zone   | M    | $\sigma_M$ | RA          | Dec        | F275   | F336   | $\sigma_{F275}$ | $\sigma_{F336}$ | x      | y      | $d_x/\sigma_x$ | Age  | $\log(T)$ | $\log(g)$ | $\sigma_{Age}$ | $\sigma_{\log T}$ | $\sigma_{\log g}$ |
|-----|--------|------|------------|-------------|------------|--------|--------|-----------------|-----------------|--------|--------|----------------|------|-----------|-----------|----------------|-------------------|-------------------|
| 21  | MS     | 21.6 | 2.4        | 152.770254  | -4.7044626 | 18.772 | 19.356 | 0.016           | 0.015           | -0.657 | -7.242 | -              | 7.8  | 4.52      | 3.78      | 1.6            | 0.05              | 0.16              |
| 22  | ZAMS.L | 21.4 | 3.7        | 152.7325566 | -4.7146808 | 19.972 | 20.588 | 0.022           | 0.017           | -0.689 | -6.042 | 1.03           | 0    | 4.6       | 4.42      | 4.6            | 0.05              | 0.18              |
| 23  | ZAMS.L | 21.3 | 3.6        | 152.7722394 | -4.702848  | 19.977 | 20.598 | 0.025           | 0.023           | -0.694 | -6.037 | 1.11           | 0    | 4.6       | 4.42      | 4.6            | 0.05              | 0.18              |
| 24  | TAMS.R | 21.2 | 2.8        | 152.7688343 | -4.7053884 | 18.506 | 19.044 | 0.025           | 0.02            | -0.611 | -7.508 | 1.03           | 8.8  | 4.48      | 3.55      | 2.2            | 0.04              | 0.16              |
| 25  | MS     | 21   | 2.4        | 152.7430348 | -4.6708346 | 18.64  | 19.21  | 0.026           | 0.014           | -0.643 | -7.374 | -              | 8.6  | 4.49      | 3.63      | 1.7            | 0.05              | 0.19              |
| 26  | MS     | 20.9 | 6.4        | 152.7242262 | -4.698985  | 19.247 | 19.839 | 0.032           | 0.028           | -0.665 | -6.767 | -              | 6.3  | 4.56      | 4.04      | 5              | 0.09              | 0.32              |
| 27  | ZAMS.L | 20.9 | 2.8        | 152.7227256 | -4.6881828 | 20.016 | 20.655 | 0.025           | 0.02            | -0.712 | -5.998 | 1.83           | 0    | 4.59      | 4.42      | 3.7            | 0.04              | 0.14              |
| 28  | TAMS.R | 20.7 | 2.3        | 152.7246998 | -4.6861546 | 18.571 | 19.132 | 0.021           | 0.016           | -0.634 | -7.443 | 0.04           | 9.1  | 4.48      | 3.55      | 1.8            | 0.04              | 0.14              |
| 29  | MS     | 20.6 | 3.8        | 152.7267779 | -4.6872964 | 19.008 | 19.595 | 0.021           | 0.019           | -0.66  | -7.006 | -              | 7.6  | 4.53      | 3.88      | 2.9            | 0.07              | 0.24              |
| 30  | ZAMS.L | 20.3 | 4          | 152.7251732 | -4.6808529 | 20.063 | 20.665 | 0.016           | 0.018           | -0.675 | -5.951 | 0.5            | 0    | 4.59      | 4.42      | 5.8            | 0.06              | 0.22              |
| 31  | MS     | 20   | 3.8        | 152.7436029 | -4.681217  | 19.092 | 19.678 | 0.021           | 0.023           | -0.659 | -6.922 | -              | 7.8  | 4.53      | 3.9       | 3.6            | 0.07              | 0.26              |
| 32  | TAMS.R | 19.1 | 1.8        | 152.7727758 | -4.700828  | 18.724 | 19.247 | 0.017           | 0.021           | -0.596 | -7.29  | 1.47           | 9.9  | 4.46      | 3.54      | 1.7            | 0.03              | 0.13              |
| 33  | MS     | 18.9 | 4.7        | 152.7272036 | -4.6872889 | 20.139 | 20.734 | 0.019           | 0.02            | -0.668 | -5.875 | 0.05           | 0.3  | 4.57      | 4.39      | 8.6            | 0.07              | 0.3               |
| 34  | ZAMS.L | 18.6 | 3          | 152.7291518 | -4.6884885 | 20.232 | 20.829 | 0.018           | 0.013           | -0.67  | -5.782 | 0.24           | 0.1  | 4.58      | 4.43      | 5.5            | 0.05              | 0.19              |
| 35  | MS     | 18.4 | 4.7        | 152.7268748 | -4.6799604 | 19.421 | 20.008 | 0.022           | 0.019           | -0.66  | -6.593 | -              | 7.8  | 4.53      | 4         | 5.4            | 0.09              | 0.3               |
| 36  | ZAMS.L | 18.3 | 2.2        | 152.7296023 | -4.6881726 | 20.264 | 20.87  | 0.017           | 0.014           | -0.679 | -5.75  | 0.79           | 0.1  | 4.57      | 4.43      | 4.1            | 0.03              | 0.13              |
| 37  | ZAMS.L | 18.1 | 3.1        | 152.7378026 | -4.6753693 | 20.287 | 20.889 | 0.018           | 0.015           | -0.675 | -5.727 | 0.53           | 0.1  | 4.57      | 4.43      | 6.1            | 0.05              | 0.2               |
| 38  | ZAMS.L | 18   | 3.1        | 152.7241693 | -4.6995356 | 20.298 | 20.906 | 0.024           | 0.022           | -0.681 | -5.716 | 0.65           | 0.1  | 4.57      | 4.43      | 6.4            | 0.05              | 0.21              |
| 39  | MS     | 17.9 | 7.4        | 152.7257461 | -4.6877296 | 19.699 | 20.289 | 0.023           | 0.022           | -0.663 | -6.315 | -              | 6.6  | 4.54      | 4.13      | 9.6            | 0.12              | 0.44              |
| 40  | ZAMS.L | 17.9 | 2.6        | 152.739362  | -4.7013478 | 20.314 | 20.923 | 0.024           | 0.024           | -0.682 | -5.7   | 0.69           | 0.1  | 4.57      | 4.43      | 5.5            | 0.04              | 0.18              |
| 41  | MS     | 17.7 | 3.6        | 152.7394993 | -4.6765679 | 19.503 | 20.088 | 0.022           | 0.024           | -0.658 | -6.511 | -              | 8.2  | 4.53      | 4         | 4.8            | 0.07              | 0.27              |
| 42  | MS     | 17.6 | 3.1        | 152.7301797 | -4.6881895 | 20.218 | 20.81  | 0.022           | 0.017           | -0.665 | -5.796 | -              | 1.6  | 4.56      | 4.36      | 6.4            | 0.05              | 0.21              |
| 43  | MS     | 17.4 | 2.8        | 152.7408959 | -4.6752623 | 20.298 | 20.89  | 0.018           | 0.016           | -0.665 | -5.716 | -              | 0.5  | 4.56      | 4.38      | 6.4            | 0.05              | 0.19              |
| 44  | MS     | 17.3 | 5.9        | 152.7246017 | -4.6864364 | 19.792 | 20.381 | 0.017           | 0.021           | -0.662 | -6.222 | -              | 6.7  | 4.54      | 4.14      | 8.7            | 0.1               | 0.38              |
| 45  | ZAMS.L | 17.1 | 1.1        | 152.7502954 | -4.6956246 | 20.403 | 21.059 | 0.033           | 0.021           | -0.729 | -5.611 | 1.93           | 0.1  | 4.56      | 4.43      | 2.5            | 0.02              | 0.07              |
| 46  | ZAMS.L | 16.7 | 5.9        | 152.7423789 | -4.6851065 | 20.45  | 21.049 | 0.022           | 0.015           | -0.672 | -5.564 | 0.32           | 0.1  | 4.56      | 4.43      | 6.5            | 0.19              | 0.56              |
| 47  | ZAMS.L | 16.5 | 2.7        | 152.7228232 | -4.6866387 | 20.485 | 21.089 | 0.031           | 0.027           | -0.677 | -5.529 | 0.39           | 0.1  | 4.56      | 4.43      | 7.1            | 0.05              | 0.21              |
| 48  | MS     | 16.3 | 5.2        | 152.7275946 | -4.6852879 | 20.135 | 20.724 | 0.021           | 0.017           | -0.662 | -5.879 | -              | 5.1  | 4.54      | 4.25      | 9.8            | 0.09              | 0.34              |
| 49  | MS     | 16.3 | 5.6        | 152.773721  | -4.7029891 | 19.842 | 20.426 | 0.032           | 0.04            | -0.657 | -6.172 | -              | 8    | 4.52      | 4.09      | 9.6            | 0.12              | 0.46              |
| 50  | MS     | 16   | 1.9        | 152.7714698 | -4.7044767 | 19.517 | 20.084 | 0.025           | 0.029           | -0.64  | -6.497 | -              | 10.6 | 4.48      | 3.85      | 2.9            | 0.06              | 0.21              |
| 51  | MS     | 16   | 1.8        | 152.7681325 | -4.70576   | 19.661 | 20.236 | 0.014           | 0.022           | -0.648 | -6.353 | -              | 9.8  | 4.5       | 3.95      | 3.1            | 0.05              | 0.19              |
| 52  | MS     | 16   | 5.8        | 152.7228914 | -4.6997977 | 20.314 | 20.903 | 0.02            | 0.02            | -0.662 | -5.7   | -              | 3.6  | 4.54      | 4.31      | 12.1           | 0.09              | 0.36              |
| 53  | ZAMS.L | 15.9 | 4.7        | 152.7499981 | -4.6645922 | 20.558 | 21.156 | 0.038           | 0.022           | -0.671 | -5.456 | 0.18           | 0.1  | 4.55      | 4.44      | 5.9            | 0.18              | 0.55              |
| 54  | TAMS.R | 15.8 | 1.8        | 152.7684158 | -4.70581   | 19.186 | 19.671 | 0.03            | 0.03            | -0.558 | -6.828 | 1.61           | 12.3 | 4.43      | 3.57      | 3.1            | 0.04              | 0.15              |
| 55  | ZAMS.L | 15.7 | 2.9        | 152.7331372 | -4.6861164 | 20.585 | 21.178 | 0.019           | 0.025           | -0.666 | -5.429 | 0.09           | 0.1  | 4.55      | 4.44      | 3.9            | 0.12              | 0.37              |
| 56  | MS     | 15.7 | 4.1        | 152.7406419 | -4.7159007 | 20.066 | 20.651 | 0.021           | 0.026           | -0.658 | -5.948 | -              | 7.1  | 4.53      | 4.17      | 8.6            | 0.08              | 0.33              |
| 57  | MS     | 15.6 | 1.2        | 152.7301871 | -4.6880928 | 19.239 | 19.771 | 0.019           | 0.019           | -0.605 | -6.775 | -              | 12.6 | 4.43      | 3.58      | 2              | 0.02              | 0.1               |
| 58  | ZAMS.L | 15.5 | 2.7        | 152.7399919 | -4.6774771 | 20.616 | 21.208 | 0.022           | 0.015           | -0.665 | -5.398 | 0.07           | 0.1  | 4.55      | 4.44      | 3.4            | 0.11              | 0.32              |
| 59  | ZAMS.L | 15.3 | 2.8        | 152.7245867 | -4.6860509 | 20.651 | 21.266 | 0.017           | 0.028           | -0.688 | -5.363 | 0.9            | 0.1  | 4.54      | 4.44      | 4              | 0.12              | 0.37              |
| 60  | ZAMS.L | 15.3 | 2.1        | 152.7277293 | -4.6818358 | 20.656 | 21.255 | 0.02            | 0.013           | -0.672 | -5.358 | 0.46           | 0.1  | 4.54      | 4.44      | 2.8            | 0.08              | 0.26              |
| 61  | MS     | 15   | 4.3        | 152.7741579 | -4.7012238 | 20.441 | 21.027 | 0.021           | 0.019           | -0.659 | -5.573 | -              | 4.2  | 4.53      | 4.31      | 12.5           | 0.07              | 0.31              |
| 62  | MS     | 15   | 2.5        | 152.747553  | -4.710203  | 20.615 | 21.202 | 0.032           | 0.025           | -0.66  | -5.399 | -              | 1.4  | 4.53      | 4.39      | 8.8            | 0.06              | 0.24              |
| 63  | ZAMS.L | 14.9 | 3.4        | 152.7167048 | -4.6858602 | 20.715 | 21.343 | 0.044           | 0.018           | -0.701 | -5.299 | 0.89           | 0.1  | 4.54      | 4.44      | 5              | 0.16              | 0.52              |
| 64  | MS     | 14.8 | 0.9        | 152.7445128 | -4.6678383 | 19.682 | 20.24  | 0.016           | 0.02            | -0.631 | -6.332 | -              | 11.8 | 4.47      | 3.83      | 1.8            | 0.03              | 0.12              |
| 65  | MS     | 14.8 | 2.9        | 152.7672028 | -4.7051815 | 20.355 | 20.939 | 0.016           | 0.018           | -0.657 | -5.659 | -              | 5.9  | 4.52      | 4.25      | 8.8            | 0.05              | 0.23              |

| IDN | Zone   | M    | $\sigma_M$ | RA          | Dec        | F275   | F336   | $\sigma_{F275}$ | $\sigma_{F336}$ | x      | y      | $d_x/\sigma_x$ | Age  | log(T) | log(g) | $\sigma_{Age}$ | $\sigma_{logT}$ | $\sigma_{logg}$ |
|-----|--------|------|------------|-------------|------------|--------|--------|-----------------|-----------------|--------|--------|----------------|------|--------|--------|----------------|-----------------|-----------------|
| 66  | ZAMS_L | 14.8 | 2.6        | 152.7390166 | -4.6747359 | 20.728 | 21.373 | 0.033           | 0.014           | -0.718 | -5.286 | 1.71           | 0.1  | 4.54   | 4.44   | 3.8            | 0.12            | 0.39            |
| 67  | MS     | 14.8 | 1.8        | 152.7437679 | -4.6774026 | 19.751 | 20.313 | 0.03            | 0.019           | -0.635 | -6.263 | -              | 11.6 | 4.48   | 3.88   | 3.9            | 0.05            | 0.19            |
| 68  | MS     | 14.7 | 1.3        | 152.7425487 | -4.6765523 | 19.391 | 19.919 | 0.018           | 0.015           | -0.601 | -6.623 | -              | 13.4 | 4.43   | 3.6    | 2.6            | 0.02            | 0.09            |
| 69  | MS     | 14.7 | 2.8        | 152.7429765 | -4.6777518 | 20.207 | 20.787 | 0.023           | 0.02            | -0.653 | -5.807 | -              | 8.1  | 4.51   | 4.16   | 7.7            | 0.06            | 0.24            |
| 70  | TAMS_R | 14.6 | 2          | 152.7292657 | -4.6991946 | 19.454 | 19.977 | 0.02            | 0.022           | -0.596 | -6.56  | 0.39           | 13.3 | 4.43   | 3.63   | 4.4            | 0.03            | 0.14            |
| 71  | MS     | 14.5 | 1.2        | 152.7343637 | -4.6742939 | 19.646 | 20.192 | 0.028           | 0.023           | -0.619 | -6.368 | -              | 12.8 | 4.45   | 3.76   | 2.4            | 0.04            | 0.14            |
| 72  | MS     | 14.4 | 4.5        | 152.7701722 | -4.7044576 | 20.673 | 21.258 | 0.017           | 0.021           | -0.658 | -5.341 | -              | 2.1  | 4.53   | 4.38   | 13.6           | 0.07            | 0.32            |
| 73  | MS     | 14.3 | 4.9        | 152.7205081 | -4.6940509 | 20.778 | 21.363 | 0.023           | 0.02            | -0.658 | -5.236 | -              | 0.5  | 4.53   | 4.41   | 13.9           | 0.07            | 0.34            |
| 74  | MS     | 14.3 | 1.1        | 152.7299629 | -4.6765314 | 19.788 | 20.343 | 0.023           | 0.021           | -0.628 | -6.226 | -              | 12.4 | 4.46   | 3.85   | 2.4            | 0.04            | 0.13            |
| 75  | MS     | 14.3 | 1.1        | 152.7275364 | -4.6991592 | 19.553 | 20.086 | 0.02            | 0.018           | -0.606 | -6.461 | -              | 13.7 | 4.43   | 3.67   | 2.5            | 0.03            | 0.1             |
| 76  | ZAMS_L | 14.2 | 2.3        | 152.7239644 | -4.6988576 | 20.827 | 21.416 | 0.035           | 0.022           | -0.662 | -5.187 | 0.07           | 0.1  | 4.53   | 4.45   | 4              | 0.12            | 0.38            |
| 77  | ZAMS_L | 14.2 | 1.7        | 152.7518263 | -4.7137485 | 20.836 | 21.454 | 0.032           | 0.033           | -0.691 | -5.178 | 0.95           | 0.1  | 4.53   | 4.45   | 3.8            | 0.1             | 0.34            |
| 78  | MS     | 14.2 | 0.7        | 152.7294363 | -4.6961575 | 19.797 | 20.35  | 0.015           | 0.018           | -0.626 | -6.217 | -              | 12.7 | 4.46   | 3.84   | 1.8            | 0.03            | 0.1             |
| 79  | MS     | 14.1 | 3.6        | 152.7402952 | -4.6763467 | 20.62  | 21.203 | 0.022           | 0.022           | -0.656 | -5.394 | -              | 4.1  | 4.52   | 4.33   | 12.5           | 0.06            | 0.29            |
| 80  | MS     | 14.1 | 1.8        | 152.7285655 | -4.6868139 | 20.015 | 20.581 | 0.028           | 0.016           | -0.639 | -5.999 | -              | 11.4 | 4.48   | 3.99   | 4.6            | 0.05            | 0.2             |
| 81  | MS     | 14   | 2.9        | 152.770848  | -4.7041261 | 20.467 | 21.047 | 0.023           | 0.015           | -0.653 | -5.547 | -              | 6.9  | 4.51   | 4.24   | 9.3            | 0.06            | 0.25            |
| 82  | MS     | 14   | 0.8        | 152.7684834 | -4.703716  | 19.768 | 20.314 | 0.02            | 0.019           | -0.619 | -6.246 | -              | 13.2 | 4.45   | 3.79   | 1.9            | 0.03            | 0.1             |
| 83  | ZAMS_L | 13.9 | 1.2        | 152.7260304 | -4.6863509 | 20.883 | 21.506 | 0.022           | 0.02            | -0.696 | -5.131 | 1.7            | 0.1  | 4.53   | 4.45   | 2.5            | 0.07            | 0.22            |
| 84  | MS     | 13.9 | 2.2        | 152.7393944 | -4.675344  | 20.154 | 20.724 | 0.028           | 0.018           | -0.643 | -5.86  | -              | 10.7 | 4.49   | 4.06   | 5.6            | 0.06            | 0.21            |
| 85  | MS     | 13.8 | 2.7        | 152.7247261 | -4.6864129 | 20.492 | 21.071 | 0.022           | 0.015           | -0.652 | -5.522 | -              | 7.1  | 4.51   | 4.24   | 8.6            | 0.06            | 0.23            |
| 86  | MS     | 13.8 | 2          | 152.7299852 | -4.6836085 | 20.043 | 20.606 | 0.032           | 0.016           | -0.636 | -5.971 | -              | 11.9 | 4.48   | 3.97   | 5              | 0.06            | 0.22            |
| 87  | MS     | 13.7 | 0.7        | 152.7277043 | -4.6847854 | 19.726 | 20.258 | 0.02            | 0.022           | -0.605 | -6.288 | -              | 14.3 | 4.43   | 3.71   | 1.7            | 0.03            | 0.1             |
| 88  | MS     | 13.7 | 2.8        | 152.7258794 | -4.6862979 | 20.579 | 21.158 | 0.023           | 0.021           | -0.652 | -5.435 | -              | 6.5  | 4.51   | 4.27   | 9.7            | 0.06            | 0.25            |
| 89  | MS     | 13.6 | 0.6        | 152.7395633 | -4.6763742 | 19.818 | 20.357 | 0.016           | 0.016           | -0.612 | -6.196 | -              | 14   | 4.44   | 3.77   | 1.4            | 0.02            | 0.08            |
| 90  | MS     | 13.5 | 1.4        | 152.7236696 | -4.6891996 | 20.276 | 20.845 | 0.02            | 0.017           | -0.642 | -5.738 | -              | 10.7 | 4.49   | 4.08   | 4.1            | 0.04            | 0.15            |
| 91  | MS     | 13.5 | 2.1        | 152.7519276 | -4.7115537 | 20.254 | 20.822 | 0.03            | 0.024           | -0.641 | -5.76  | -              | 11   | 4.49   | 4.07   | 6.2            | 0.06            | 0.21            |
| 92  | ZAMS_L | 13.5 | 1.2        | 152.7344549 | -4.6837632 | 20.962 | 21.578 | 0.029           | 0.02            | -0.689 | -5.052 | 1.11           | 0.1  | 4.52   | 4.45   | 2.9            | 0.08            | 0.27            |
| 93  | ZAMS_L | 13.3 | 1.6        | 152.7583805 | -4.6964503 | 21.002 | 21.632 | 0.048           | 0.028           | -0.703 | -5.012 | 0.98           | 0.1  | 4.52   | 4.45   | 4.3            | 0.13            | 0.41            |
| 94  | TAMS_R | 13.3 | 1          | 152.7265178 | -4.6889092 | 19.657 | 20.162 | 0.02            | 0.019           | -0.578 | -6.357 | 0.44           | 15.6 | 4.41   | 3.61   | 2.7            | 0.02            | 0.1             |
| 95  | MS     | 13.3 | 4.5        | 152.7486872 | -4.6732668 | 20.949 | 21.529 | 0.021           | 0.029           | -0.653 | -5.065 | -              | 1.3  | 4.51   | 4.41   | 15.6           | 0.08            | 0.37            |
| 96  | MS     | 13.2 | 1.2        | 152.7561823 | -4.7085888 | 20.067 | 20.62  | 0.026           | 0.028           | -0.626 | -5.947 | -              | 13.3 | 4.46   | 3.92   | 3.5            | 0.04            | 0.17            |
| 97  | MS     | 13.2 | 0.9        | 152.7241716 | -4.6882851 | 19.809 | 20.337 | 0.016           | 0.029           | -0.601 | -6.205 | -              | 14.9 | 4.43   | 3.72   | 2.3            | 0.04            | 0.13            |
| 98  | TAMS_R | 13.2 | 0.9        | 152.7436219 | -4.6780186 | 19.67  | 20.168 | 0.018           | 0.014           | -0.571 | -6.344 | 0.85           | 15.7 | 4.41   | 3.61   | 2.4            | 0.02            | 0.09            |
| 99  | ZAMS_L | 13.2 | 0.8        | 152.7230203 | -4.6868715 | 21.016 | 21.615 | 0.026           | 0.026           | -0.672 | -4.998 | 0.63           | 0.1  | 4.52   | 4.45   | 2.4            | 0.07            | 0.23            |
| 100 | MS     | 13.2 | 2.4        | 152.7233208 | -4.6948618 | 20.518 | 21.091 | 0.027           | 0.026           | -0.646 | -5.496 | -              | 9    | 4.5    | 4.19   | 8.2            | 0.06            | 0.23            |
| 101 | ZAMS_L | 13.2 | 0.6        | 152.7309929 | -4.6860052 | 21.019 | 21.62  | 0.017           | 0.019           | -0.674 | -4.995 | 0.97           | 0.1  | 4.52   | 4.45   | 1.8            | 0.05            | 0.17            |
| 102 | ZAMS_L | 13.2 | 0.9        | 152.7279534 | -4.6863398 | 21.02  | 21.611 | 0.028           | 0.017           | -0.664 | -4.994 | 0.3            | 0.1  | 4.52   | 4.45   | 2.5            | 0.07            | 0.24            |
| 103 | MS     | 13.1 | 1.9        | 152.7264185 | -4.6891659 | 20.183 | 20.741 | 0.036           | 0.023           | -0.631 | -5.831 | -              | 12.7 | 4.47   | 3.98   | 5.6            | 0.06            | 0.22            |
| 104 | TAMS_R | 13.1 | 1.4        | 152.7449824 | -4.6857089 | 19.692 | 20.203 | 0.027           | 0.018           | -0.584 | -6.322 | 0.05           | 15.9 | 4.41   | 3.61   | 3.6            | 0.03            | 0.13            |
| 105 | ZAMS_L | 13.1 | 0.7        | 152.7341406 | -4.6813811 | 21.044 | 21.633 | 0.022           | 0.024           | -0.662 | -4.97  | 0.29           | 0.1  | 4.52   | 4.45   | 2.2            | 0.06            | 0.21            |
| 106 | MS     | 13   | 2.2        | 152.7266887 | -4.6860786 | 20.684 | 21.259 | 0.021           | 0.018           | -0.648 | -5.33  | -              | 7.2  | 4.5    | 4.26   | 7.8            | 0.05            | 0.2             |
| 107 | MS     | 13   | 2.3        | 152.7546054 | -4.6743987 | 20.407 | 20.974 | 0.032           | 0.036           | -0.64  | -5.607 | -              | 10.9 | 4.48   | 4.11   | 8              | 0.07            | 0.26            |
| 108 | ZAMS_L | 13   | 0.5        | 152.7702324 | -4.701308  | 21.059 | 21.65  | 0.02            | 0.018           | -0.664 | -4.955 | 0.47           | 0.1  | 4.52   | 4.45   | 1.6            | 0.05            | 0.16            |
| 109 | ZAMS_L | 12.9 | 0.7        | 152.7530898 | -4.6737595 | 21.069 | 21.666 | 0.024           | 0.031           | -0.67  | -4.945 | 0.5            | 0.1  | 4.51   | 4.45   | 2.6            | 0.08            | 0.26            |
| 110 | ZAMS_L | 12.9 | 0.5        | 152.7342778 | -4.6737163 | 21.079 | 21.684 | 0.02            | 0.02            | -0.678 | -4.935 | 1.19           | 0.1  | 4.51   | 4.45   | 1.7            | 0.05            | 0.17            |

| IDN | Zone   | M    | $\sigma_M$ | RA          | Dec        | F275   | F336   | $\sigma_{F275}$ | $\sigma_{F336}$ | x      | y      | $d_x/\sigma_x$ | Age  | log(T) | log(g) | $\sigma_{Age}$ | $\sigma_{logT}$ | $\sigma_{logg}$ |
|-----|--------|------|------------|-------------|------------|--------|--------|-----------------|-----------------|--------|--------|----------------|------|--------|--------|----------------|-----------------|-----------------|
| 111 | MS     | 12.9 | 0.7        | 152.7262125 | -4.6893519 | 20.03  | 20.57  | 0.021           | 0.014           | -0.613 | -5.984 | -              | 14.6 | 4.44   | 3.84   | 2.2            | 0.03            | 0.1             |
| 112 | MS     | 12.9 | 1.9        | 152.7410972 | -4.6698397 | 20.716 | 21.29  | 0.02            | 0.018           | -0.647 | -5.298 | -              | 7.4  | 4.5    | 4.26   | 7.4            | 0.04            | 0.18            |
| 113 | MS     | 12.8 | 1          | 152.7240171 | -4.6998586 | 20.161 | 20.711 | 0.024           | 0.021           | -0.623 | -5.853 | -              | 13.8 | 4.46   | 3.93   | 3.1            | 0.04            | 0.13            |
| 114 | MS     | 12.7 | 1          | 152.7313734 | -4.6957593 | 20.354 | 20.914 | 0.019           | 0.016           | -0.633 | -5.66  | -              | 12.4 | 4.47   | 4.04   | 3.5            | 0.03            | 0.12            |
| 115 | MS     | 12.7 | 1.4        | 152.7240296 | -4.6987543 | 20.631 | 21.201 | 0.018           | 0.017           | -0.643 | -5.383 | -              | 9.3  | 4.49   | 4.2    | 5.6            | 0.04            | 0.14            |
| 116 | MS     | 12.7 | 1.3        | 152.7236125 | -4.6884484 | 19.937 | 20.461 | 0.042           | 0.036           | -0.597 | -6.077 | -              | 15.7 | 4.42   | 3.73   | 3.8            | 0.05            | 0.18            |
| 117 | MS     | 12.7 | 0.7        | 152.7456768 | -4.7023311 | 20.069 | 20.606 | 0.016           | 0.022           | -0.61  | -5.945 | -              | 15   | 4.44   | 3.83   | 2.2            | 0.03            | 0.11            |
| 118 | MS     | 12.7 | 1          | 152.7374137 | -4.6751369 | 20.529 | 21.095 | 0.015           | 0.016           | -0.639 | -5.485 | -              | 10.9 | 4.48   | 4.14   | 3.8            | 0.03            | 0.12            |
| 119 | MS     | 12.6 | 1.2        | 152.7257924 | -4.6882969 | 20.332 | 20.889 | 0.021           | 0.025           | -0.63  | -5.682 | -              | 13   | 4.47   | 4.02   | 4.1            | 0.04            | 0.15            |
| 120 | MS     | 12.6 | 1.7        | 152.7232346 | -4.6875469 | 20.555 | 21.121 | 0.022           | 0.026           | -0.639 | -5.459 | -              | 10.8 | 4.48   | 4.15   | 6.7            | 0.05            | 0.19            |
| 121 | MS     | 12.5 | 1.5        | 152.75373   | -4.681901  | 20.499 | 21.062 | 0.018           | 0.024           | -0.636 | -5.515 | -              | 11.6 | 4.48   | 4.11   | 5.3            | 0.04            | 0.17            |
| 122 | MS     | 12.5 | 1.1        | 152.7643971 | -4.7076958 | 20.485 | 21.047 | 0.015           | 0.019           | -0.635 | -5.529 | -              | 11.9 | 4.48   | 4.1    | 3.9            | 0.03            | 0.13            |
| 123 | ZAMS_L | 12.5 | 0.7        | 152.75679   | -4.6921957 | 21.167 | 21.75  | 0.026           | 0.016           | -0.656 | -4.847 | 0.16           | 0.1  | 4.51   | 4.46   | 1.9            | 0.06            | 0.2             |
| 124 | ZAMS_L | 12.5 | 1.1        | 152.7251797 | -4.6987589 | 21.167 | 21.755 | 0.044           | 0.026           | -0.661 | -4.847 | 0.21           | 0.1  | 4.51   | 4.46   | 3.3            | 0.1             | 0.33            |
| 125 | MS     | 12.5 | 0.7        | 152.7313228 | -4.6857694 | 20.134 | 20.672 | 0.019           | 0.021           | -0.611 | -5.88  | -              | 15.1 | 4.44   | 3.86   | 2.2            | 0.03            | 0.11            |
| 126 | MS     | 12.5 | 3.1        | 152.7538573 | -4.6911409 | 20.947 | 21.521 | 0.029           | 0.022           | -0.647 | -5.067 | -              | 4.9  | 4.5    | 4.34   | 14.1           | 0.06            | 0.28            |
| 127 | MS     | 12.5 | 0.6        | 152.7280299 | -4.7000133 | 20.08  | 20.612 | 0.017           | 0.018           | -0.605 | -5.934 | -              | 15.6 | 4.43   | 3.81   | 1.7            | 0.02            | 0.09            |
| 128 | MS     | 12.5 | 2.1        | 152.7545862 | -4.7082998 | 20.477 | 21.038 | 0.026           | 0.038           | -0.634 | -5.537 | -              | 12.1 | 4.47   | 4.09   | 7.8            | 0.07            | 0.26            |
| 129 | MS     | 12.5 | 0.6        | 152.7317697 | -4.6863766 | 20.099 | 20.632 | 0.018           | 0.017           | -0.606 | -5.915 | -              | 15.5 | 4.43   | 3.82   | 1.8            | 0.02            | 0.08            |
| 130 | MS     | 12.5 | 2.5        | 152.7316267 | -4.7148468 | 20.974 | 21.548 | 0.018           | 0.025           | -0.647 | -5.04  | -              | 4.6  | 4.5    | 4.35   | 13             | 0.05            | 0.24            |
| 131 | MS     | 12.4 | 1.5        | 152.7220695 | -4.6861758 | 20.538 | 21.101 | 0.024           | 0.026           | -0.636 | -5.476 | -              | 11.6 | 4.48   | 4.12   | 5.8            | 0.05            | 0.18            |
| 132 | MS     | 12.4 | 1.7        | 152.7245858 | -4.686092  | 20.696 | 21.264 | 0.023           | 0.023           | -0.641 | -5.318 | -              | 9.6  | 4.49   | 4.2    | 7.3            | 0.04            | 0.18            |
| 133 | MS     | 12.4 | 1.3        | 152.7289706 | -4.6853608 | 20.535 | 21.097 | 0.021           | 0.014           | -0.635 | -5.479 | -              | 11.8 | 4.48   | 4.11   | 4.7            | 0.04            | 0.14            |
| 134 | ZAMS_L | 12.4 | 0.6        | 152.734237  | -4.6757395 | 21.194 | 21.82  | 0.024           | 0.024           | -0.699 | -4.82  | 1.99           | 0.1  | 4.51   | 4.46   | 1.8            | 0.06            | 0.19            |
| 135 | MS     | 12.4 | 1.2        | 152.7343998 | -4.713527  | 20.126 | 20.659 | 0.038           | 0.018           | -0.606 | -5.888 | -              | 15.6 | 4.43   | 3.83   | 3.9            | 0.05            | 0.17            |
| 136 | MS     | 12.4 | 0.6        | 152.7291229 | -4.6985466 | 20.109 | 20.64  | 0.018           | 0.012           | -0.604 | -5.905 | -              | 15.8 | 4.43   | 3.81   | 1.8            | 0.02            | 0.08            |
| 137 | MS     | 12.4 | 0.7        | 152.7343437 | -4.7015192 | 19.977 | 20.493 | 0.017           | 0.023           | -0.589 | -6.037 | -              | 16.6 | 4.41   | 3.71   | 2              | 0.03            | 0.1             |
| 138 | MS     | 12.3 | 0.7        | 152.7287789 | -4.6846663 | 20.321 | 20.87  | 0.017           | 0.019           | -0.622 | -5.693 | -              | 14.2 | 4.46   | 3.97   | 2.6            | 0.03            | 0.11            |
| 139 | MS     | 12.3 | 2.2        | 152.727317  | -4.6969601 | 20.872 | 21.443 | 0.025           | 0.017           | -0.644 | -5.142 | -              | 7.2  | 4.49   | 4.29   | 10.3           | 0.05            | 0.21            |
| 140 | MS     | 12.3 | 0.8        | 152.7297257 | -4.6983669 | 20.216 | 20.755 | 0.024           | 0.018           | -0.612 | -5.798 | -              | 15.3 | 4.44   | 3.88   | 2.7            | 0.03            | 0.12            |
| 141 | ZAMS_L | 12.3 | 1          | 152.7239889 | -4.6992658 | 21.216 | 21.811 | 0.041           | 0.02            | -0.668 | -4.798 | 0.43           | 0.1  | 4.51   | 4.46   | 2.8            | 0.09            | 0.29            |
| 142 | MS     | 12.3 | 1          | 152.7254602 | -4.6919302 | 20.254 | 20.796 | 0.028           | 0.019           | -0.615 | -5.76  | -              | 15   | 4.45   | 3.91   | 3.3            | 0.04            | 0.14            |
| 143 | MS     | 12.3 | 0.7        | 152.7539274 | -4.6803724 | 20.032 | 20.551 | 0.024           | 0.022           | -0.592 | -5.982 | -              | 16.6 | 4.42   | 3.74   | 2.3            | 0.03            | 0.1             |
| 144 | MS     | 12.3 | 0.8        | 152.7704666 | -4.6984427 | 21.206 | 21.781 | 0.03            | 0.02            | -0.648 | -4.808 | -              | 0.3  | 4.5    | 4.44   | 2.2            | 0.07            | 0.22            |
| 145 | ZAMS_L | 12.3 | 0.9        | 152.7236231 | -4.6946263 | 21.221 | 21.867 | 0.036           | 0.028           | -0.719 | -4.793 | 1.91           | 0.1  | 4.5    | 4.46   | 2.5            | 0.08            | 0.26            |
| 146 | MS     | 12.2 | 0.7        | 152.7515744 | -4.7051241 | 20.208 | 20.744 | 0.022           | 0.018           | -0.609 | -5.806 | -              | 15.6 | 4.44   | 3.87   | 2.4            | 0.03            | 0.1             |
| 147 | MS     | 12.2 | 2.4        | 152.7483987 | -4.6670138 | 20.769 | 21.336 | 0.032           | 0.023           | -0.64  | -5.245 | -              | 9.5  | 4.48   | 4.22   | 9.6            | 0.06            | 0.24            |
| 148 | MS     | 12.2 | 1.7        | 152.7384438 | -4.6748696 | 20.792 | 21.359 | 0.021           | 0.022           | -0.64  | -5.222 | -              | 9.3  | 4.48   | 4.23   | 7.4            | 0.04            | 0.18            |
| 149 | MS     | 12.1 | 0.6        | 152.7189643 | -4.6942333 | 20.102 | 20.624 | 0.02            | 0.021           | -0.595 | -5.912 | -              | 16.6 | 4.42   | 3.77   | 2              | 0.03            | 0.1             |
| 150 | MS     | 12.1 | 1.2        | 152.7287899 | -4.6853583 | 20.499 | 21.054 | 0.024           | 0.025           | -0.628 | -5.515 | -              | 13.3 | 4.46   | 4.06   | 4.4            | 0.04            | 0.15            |
| 151 | MS     | 12.1 | 3.7        | 152.7380996 | -4.6746146 | 20.887 | 21.455 | 0.046           | 0.044           | -0.641 | -5.127 | -              | 8.2  | 4.49   | 4.27   | 17             | 0.09            | 0.36            |
| 152 | MS     | 12   | 0.9        | 152.7264423 | -4.6874506 | 20.478 | 21.03  | 0.021           | 0.018           | -0.625 | -5.536 | -              | 13.8 | 4.46   | 4.03   | 3.5            | 0.03            | 0.12            |
| 153 | MS     | 12   | 0.6        | 152.737517  | -4.675365  | 20.322 | 20.862 | 0.018           | 0.019           | -0.613 | -5.692 | -              | 15.4 | 4.44   | 3.92   | 2.4            | 0.03            | 0.1             |
| 154 | MS     | 11.9 | 0.7        | 152.7284286 | -4.6870728 | 20.094 | 20.607 | 0.023           | 0.012           | -0.586 | -5.92  | -              | 17.4 | 4.41   | 3.73   | 2.4            | 0.03            | 0.1             |
| 155 | MS     | 11.9 | 2.5        | 152.7284257 | -4.6906528 | 21.247 | 21.818 | 0.029           | 0.025           | -0.644 | -4.767 | -              | 1.7  | 4.49   | 4.41   | 15             | 0.06            | 0.26            |

| IDN | Zone   | M    | $\sigma_M$ | RA          | Dec        | F275   | F336   | $\sigma_{F275}$ | $\sigma_{F336}$ | x      | y      | $d_x/\sigma_x$ | Age  | log(T) | log(g) | $\sigma_{Age}$ | $\sigma_{\log T}$ | $\sigma_{\log g}$ |
|-----|--------|------|------------|-------------|------------|--------|--------|-----------------|-----------------|--------|--------|----------------|------|--------|--------|----------------|-------------------|-------------------|
| 156 | MS     | 11.9 | 1.5        | 152.7436699 | -4.6763522 | 20.589 | 21.143 | 0.034           | 0.02            | -0.627 | -5.425 | -              | 13.4 | 4.46   | 4.08   | 6.6            | 0.05              | 0.19              |
| 157 | ZAMS_L | 11.8 | 0.7        | 152.7235903 | -4.6866091 | 21.317 | 21.925 | 0.031           | 0.019           | -0.681 | -4.697 | 1.08           | 0.1  | 4.5    | 4.46   | 1.9            | 0.06              | 0.21              |
| 158 | ZAMS_L | 11.8 | 0.6        | 152.7692803 | -4.7052675 | 21.32  | 21.903 | 0.023           | 0.033           | -0.656 | -4.694 | 0.26           | 0.1  | 4.5    | 4.46   | 2.1            | 0.07              | 0.23              |
| 159 | MS     | 11.8 | 3.9        | 152.7549997 | -4.686095  | 21.162 | 21.732 | 0.042           | 0.034           | -0.643 | -4.852 | -              | 3.9  | 4.49   | 4.37   | 18.3           | 0.08              | 0.37              |
| 160 | TAMS_R | 11.8 | 0.8        | 152.7408483 | -4.6758263 | 19.98  | 20.464 | 0.018           | 0.017           | -0.557 | -6.034 | 0.86           | 18.4 | 4.39   | 3.63   | 3              | 0.02              | 0.09              |
| 161 | ZAMS_L | 11.8 | 0.7        | 152.7314809 | -4.6924795 | 21.325 | 21.907 | 0.032           | 0.027           | -0.655 | -4.689 | 0.24           | 0.1  | 4.5    | 4.46   | 2              | 0.07              | 0.21              |
| 162 | MS     | 11.8 | 1.1        | 152.7305358 | -4.6991968 | 20.493 | 21.04  | 0.029           | 0.016           | -0.62  | -5.521 | -              | 14.6 | 4.45   | 4.01   | 4.8            | 0.04              | 0.15              |
| 163 | ZAMS_L | 11.8 | 0.5        | 152.7623423 | -4.6974705 | 21.331 | 21.923 | 0.021           | 0.017           | -0.665 | -4.683 | 0.85           | 0.1  | 4.5    | 4.46   | 1.3            | 0.04              | 0.14              |
| 164 | MS     | 11.8 | 0.5        | 152.7651301 | -4.7021618 | 20.189 | 20.707 | 0.018           | 0.017           | -0.591 | -5.825 | -              | 17.3 | 4.42   | 3.78   | 1.9            | 0.02              | 0.08              |
| 165 | ZAMS_L | 11.7 | 0.7        | 152.7686181 | -4.7035254 | 21.342 | 21.964 | 0.031           | 0.017           | -0.695 | -4.672 | 1.55           | 0.1  | 4.5    | 4.46   | 1.9            | 0.06              | 0.21              |
| 166 | ZAMS_L | 11.7 | 0.7        | 152.7279094 | -4.6887741 | 21.347 | 21.926 | 0.031           | 0.016           | -0.652 | -4.667 | 0.17           | 0.1  | 4.5    | 4.46   | 1.9            | 0.06              | 0.21              |
| 167 | MS     | 11.7 | 0.4        | 152.7399558 | -4.6742219 | 20.251 | 20.773 | 0.013           | 0.016           | -0.595 | -5.763 | -              | 17.2 | 4.42   | 3.81   | 1.7            | 0.02              | 0.07              |
| 168 | MS     | 11.7 | 0.6        | 152.7400762 | -4.6760215 | 20.396 | 20.932 | 0.018           | 0.018           | -0.609 | -5.618 | -              | 16.1 | 4.44   | 3.92   | 2.3            | 0.02              | 0.09              |
| 169 | MS     | 11.7 | 0.8        | 152.7387569 | -4.675611  | 20.104 | 20.61  | 0.027           | 0.024           | -0.579 | -5.91  | -              | 18.2 | 4.4    | 3.7    | 2.9            | 0.03              | 0.12              |
| 170 | MS     | 11.7 | 0.7        | 152.7226604 | -4.6880678 | 20.537 | 21.084 | 0.019           | 0.019           | -0.62  | -5.477 | -              | 14.7 | 4.45   | 4.02   | 3.2            | 0.03              | 0.1               |
| 171 | MS     | 11.7 | 1.6        | 152.726941  | -4.6871076 | 20.974 | 21.539 | 0.019           | 0.023           | -0.638 | -5.04  | -              | 8.6  | 4.48   | 4.27   | 8.8            | 0.04              | 0.18              |
| 172 | MS     | 11.7 | 0.8        | 152.7154167 | -4.6891865 | 20.324 | 20.852 | 0.026           | 0.018           | -0.601 | -5.69  | -              | 16.8 | 4.43   | 3.86   | 3              | 0.03              | 0.12              |
| 173 | ZAMS_L | 11.7 | 0.9        | 152.7641622 | -4.7080976 | 21.364 | 21.944 | 0.042           | 0.036           | -0.653 | -4.65  | 0.16           | 0.1  | 4.5    | 4.46   | 2.6            | 0.09              | 0.28              |
| 174 | ZAMS_L | 11.7 | 0.4        | 152.7659704 | -4.7051142 | 21.363 | 21.962 | 0.02            | 0.019           | -0.672 | -4.651 | 1.29           | 0.1  | 4.5    | 4.46   | 1.2            | 0.04              | 0.13              |
| 175 | MS     | 11.6 | 0.5        | 152.7542764 | -4.7076    | 20.346 | 20.875 | 0.016           | 0.018           | -0.602 | -5.668 | -              | 16.8 | 4.43   | 3.87   | 2.1            | 0.02              | 0.09              |
| 176 | ZAMS_L | 11.6 | 0.6        | 152.7245867 | -4.688789  | 21.381 | 21.961 | 0.025           | 0.036           | -0.653 | -4.633 | 0.2            | 0.1  | 4.49   | 4.46   | 2.1            | 0.07              | 0.23              |
| 177 | ZAMS_L | 11.6 | 0.4        | 152.723713  | -4.6862501 | 21.384 | 21.977 | 0.02            | 0.022           | -0.666 | -4.63  | 0.93           | 0.1  | 4.49   | 4.46   | 1.3            | 0.04              | 0.14              |
| 178 | ZAMS_L | 11.6 | 0.5        | 152.7710514 | -4.6995288 | 21.387 | 21.969 | 0.025           | 0.022           | -0.655 | -4.627 | 0.38           | 0.1  | 4.49   | 4.46   | 1.4            | 0.05              | 0.16              |
| 179 | MS     | 11.5 | 1.1        | 152.7406646 | -4.6756793 | 20.775 | 21.331 | 0.021           | 0.017           | -0.629 | -5.239 | -              | 12.5 | 4.47   | 4.15   | 4.9            | 0.03              | 0.12              |
| 180 | MS     | 11.5 | 0.7        | 152.7311127 | -4.6952145 | 20.471 | 21.008 | 0.022           | 0.015           | -0.61  | -5.543 | -              | 16.1 | 4.44   | 3.95   | 3.1            | 0.03              | 0.11              |
| 181 | MS     | 11.5 | 1          | 152.7209668 | -4.6974558 | 20.408 | 20.939 | 0.031           | 0.028           | -0.604 | -5.606 | -              | 16.7 | 4.43   | 3.9    | 3.9            | 0.04              | 0.14              |
| 182 | MS     | 11.5 | 1.4        | 152.7410128 | -4.6757839 | 20.94  | 21.501 | 0.023           | 0.02            | -0.634 | -5.074 | -              | 10.3 | 4.47   | 4.23   | 6.8            | 0.04              | 0.15              |
| 183 | MS     | 11.4 | 1.6        | 152.7530663 | -4.6916003 | 20.112 | 20.609 | 0.026           | 0.041           | -0.57  | -5.902 | -              | 19.2 | 4.39   | 3.66   | 6.9            | 0.05              | 0.21              |
| 184 | ZAMS_L | 11.4 | 1          | 152.7747126 | -4.7023801 | 21.417 | 22.047 | 0.05            | 0.045           | -0.703 | -4.597 | 1.17           | 0.1  | 4.49   | 4.47   | 2.8            | 0.1               | 0.31              |
| 185 | TAMS_R | 11.4 | 1          | 152.7411687 | -4.7061397 | 20.083 | 20.532 | 0.023           | 0.024           | -0.522 | -5.931 | 1.91           | 19.5 | 4.39   | 3.64   | 4.1            | 0.03              | 0.12              |
| 186 | MS     | 11.4 | 1.7        | 152.7402065 | -4.6743352 | 20.989 | 21.55  | 0.027           | 0.016           | -0.634 | -5.025 | -              | 9.9  | 4.47   | 4.24   | 9              | 0.04              | 0.18              |
| 187 | MS     | 11.4 | 1.3        | 152.7671517 | -4.7004153 | 20.804 | 21.358 | 0.027           | 0.027           | -0.627 | -5.21  | -              | 12.9 | 4.46   | 4.14   | 6.6            | 0.04              | 0.16              |
| 188 | MS     | 11.4 | 0.7        | 152.7604146 | -4.7044614 | 20.582 | 21.123 | 0.02            | 0.017           | -0.614 | -5.432 | -              | 15.7 | 4.44   | 4      | 3.2            | 0.03              | 0.1               |
| 189 | MS     | 11.4 | 1.1        | 152.740332  | -4.6776117 | 20.837 | 21.392 | 0.023           | 0.018           | -0.628 | -5.177 | -              | 12.5 | 4.46   | 4.16   | 5.4            | 0.03              | 0.13              |
| 190 | MS     | 11.4 | 0.6        | 152.7683377 | -4.7056037 | 20.409 | 20.934 | 0.018           | 0.021           | -0.598 | -5.605 | -              | 17.5 | 4.42   | 3.87   | 2.4            | 0.03              | 0.1               |
| 191 | TAMS_R | 11.3 | 0.8        | 152.733428  | -4.6854736 | 20.1   | 20.564 | 0.014           | 0.019           | -0.537 | -5.914 | 1.59           | 19.6 | 4.39   | 3.64   | 3.2            | 0.02              | 0.1               |
| 192 | ZAMS_L | 11.3 | 0.5        | 152.7240434 | -4.6885467 | 21.439 | 22.011 | 0.019           | 0.028           | -0.645 | -4.575 | 0.04           | 0.1  | 4.49   | 4.47   | 1.6            | 0.06              | 0.18              |
| 193 | ZAMS_L | 11.3 | 0.5        | 152.7246878 | -4.6864002 | 21.439 | 22.014 | 0.025           | 0.016           | -0.648 | -4.575 | 0.17           | 0.1  | 4.49   | 4.47   | 1.4            | 0.05              | 0.16              |
| 194 | MS     | 11.3 | 0.7        | 152.7498418 | -4.6895022 | 20.295 | 20.807 | 0.023           | 0.016           | -0.585 | -5.719 | -              | 18.4 | 4.41   | 3.78   | 2.5            | 0.03              | 0.1               |
| 195 | ZAMS_L | 11.3 | 0.3        | 152.7495238 | -4.7038371 | 21.447 | 22.042 | 0.016           | 0.016           | -0.668 | -4.567 | 1.52           | 0.1  | 4.49   | 4.47   | 0.9            | 0.03              | 0.1               |
| 196 | MS     | 11.2 | 0.5        | 152.7660508 | -4.7028588 | 20.618 | 21.156 | 0.015           | 0.013           | -0.611 | -5.396 | -              | 16.2 | 4.44   | 4      | 2.4            | 0.02              | 0.07              |
| 197 | MS     | 11.2 | 1.1        | 152.764768  | -4.7011011 | 20.908 | 21.462 | 0.022           | 0.018           | -0.627 | -5.106 | -              | 12.5 | 4.46   | 4.17   | 5.5            | 0.03              | 0.13              |
| 198 | ZAMS_L | 11.2 | 0.7        | 152.7692378 | -4.7056714 | 21.483 | 22.059 | 0.038           | 0.016           | -0.649 | -4.531 | 0.17           | 0.1  | 4.49   | 4.47   | 1.9            | 0.07              | 0.22              |
| 199 | MS     | 11.1 | 1.1        | 152.7304224 | -4.6984585 | 20.501 | 21.026 | 0.038           | 0.019           | -0.598 | -5.513 | -              | 17.7 | 4.42   | 3.9    | 4.7            | 0.05              | 0.17              |
| 200 | TAMS_R | 11.1 | 1          | 152.7532472 | -4.6712067 | 20.158 | 20.606 | 0.023           | 0.025           | -0.521 | -5.856 | 1.74           | 20.2 | 4.38   | 3.65   | 4.5            | 0.03              | 0.13              |

| IDN | Zone   | M    | $\sigma_M$ | RA          | Dec        | F275   | F336   | $\sigma_{F275}$ | $\sigma_{F336}$ | x      | y      | $d_x/\sigma_x$ | Age  | $\log(T)$ | $\log(g)$ | $\sigma_{Age}$ | $\sigma_{\log T}$ | $\sigma_{\log g}$ |
|-----|--------|------|------------|-------------|------------|--------|--------|-----------------|-----------------|--------|--------|----------------|------|-----------|-----------|----------------|-------------------|-------------------|
| 201 | MS     | 11.1 | 0.6        | 152.7666127 | -4.7019302 | 20.356 | 20.865 | 0.02            | 0.017           | -0.582 | -5.658 | -              | 19   | 4.4       | 3.78      | 2.3            | 0.02              | 0.09              |
| 202 | TAMS.R | 11.1 | 1          | 152.7438011 | -4.6719172 | 20.165 | 20.624 | 0.023           | 0.024           | -0.532 | -5.849 | 1.34           | 20.3 | 4.38      | 3.65      | 4.4            | 0.03              | 0.12              |
| 203 | MS     | 11.1 | 0.7        | 152.7254391 | -4.6892169 | 20.583 | 21.114 | 0.023           | 0.014           | -0.604 | -5.431 | -              | 17.1 | 4.43      | 3.95      | 3.3            | 0.03              | 0.11              |
| 204 | MS     | 11   | 0.5        | 152.7455471 | -4.6670203 | 21.502 | 22.068 | 0.027           | 0.019           | -0.639 | -4.512 | -              | 0.3  | 4.48      | 4.45      | 1.4            | 0.05              | 0.16              |
| 205 | MS     | 11   | 0.7        | 152.7696648 | -4.69917   | 20.345 | 20.85  | 0.024           | 0.018           | -0.578 | -5.669 | -              | 19.4 | 4.4       | 3.76      | 2.7            | 0.03              | 0.1               |
| 206 | MS     | 11   | 2.1        | 152.7707952 | -4.704739  | 21.461 | 22.025 | 0.027           | 0.033           | -0.637 | -4.533 | -              | 1.6  | 4.48      | 4.42      | 14             | 0.06              | 0.25              |
| 207 | MS     | 11   | 1.1        | 152.7459559 | -4.6798832 | 20.67  | 21.206 | 0.032           | 0.017           | -0.609 | -5.344 | -              | 16.5 | 4.44      | 4         | 5.2            | 0.04              | 0.16              |
| 208 | MS     | 11   | 1          | 152.7295062 | -4.6863934 | 20.776 | 21.318 | 0.027           | 0.017           | -0.615 | -5.238 | -              | 15.5 | 4.45      | 4.07      | 5.2            | 0.04              | 0.14              |
| 209 | TAMS.R | 11   | 1          | 152.7598855 | -4.682919  | 20.194 | 20.675 | 0.023           | 0.025           | -0.554 | -5.82  | 0.35           | 20.6 | 4.38      | 3.65      | 4.5            | 0.03              | 0.13              |
| 210 | MS     | 11   | 1.6        | 152.7219711 | -4.6942593 | 21.077 | 21.633 | 0.029           | 0.017           | -0.629 | -4.937 | -              | 10.8 | 4.46      | 4.24      | 8.8            | 0.04              | 0.18              |
| 211 | MS     | 11   | 0.7        | 152.7308509 | -4.7098645 | 20.364 | 20.869 | 0.018           | 0.027           | -0.578 | -5.65  | -              | 19.5 | 4.4       | 3.77      | 3              | 0.03              | 0.12              |
| 212 | MS     | 11   | 0.4        | 152.72927   | -4.6875313 | 21.533 | 22.1   | 0.021           | 0.021           | -0.64  | -4.481 | -              | 0.2  | 4.48      | 4.47      | 1.1            | 0.04              | 0.13              |
| 213 | ZAMS.L | 10.9 | 0.5        | 152.7230758 | -4.6899433 | 21.54  | 22.112 | 0.027           | 0.027           | -0.645 | -4.474 | 0.17           | 0.1  | 4.48      | 4.47      | 1.3            | 0.05              | 0.15              |
| 214 | ZAMS.L | 10.9 | 0.3        | 152.7738684 | -4.7023553 | 21.546 | 22.139 | 0.017           | 0.024           | -0.666 | -4.468 | 1.07           | 0.1  | 4.48      | 4.47      | 1.2            | 0.04              | 0.14              |
| 215 | MS     | 10.9 | 0.6        | 152.7688806 | -4.7050942 | 20.69  | 21.224 | 0.017           | 0.022           | -0.607 | -5.324 | -              | 16.9 | 4.44      | 4         | 3.6            | 0.03              | 0.11              |
| 216 | MS     | 10.9 | 0.7        | 152.7747168 | -4.7019567 | 20.577 | 21.101 | 0.025           | 0.019           | -0.597 | -5.437 | -              | 18.1 | 4.42      | 3.92      | 3.5            | 0.03              | 0.11              |
| 217 | ZAMS.L | 10.9 | 0.6        | 152.7379172 | -4.6768319 | 21.549 | 22.127 | 0.038           | 0.016           | -0.651 | -4.465 | 0.29           | 0.1  | 4.48      | 4.47      | 1.8            | 0.07              | 0.21              |
| 218 | ZAMS.L | 10.9 | 0.6        | 152.7300064 | -4.6878833 | 21.551 | 22.128 | 0.034           | 0.025           | -0.65  | -4.463 | 0.29           | 0.1  | 4.48      | 4.47      | 1.6            | 0.06              | 0.18              |
| 219 | MS     | 10.9 | 1.9        | 152.7380848 | -4.6765963 | 21.135 | 21.691 | 0.037           | 0.02            | -0.629 | -4.879 | -              | 10.3 | 4.46      | 4.26      | 12.1           | 0.06              | 0.23              |
| 220 | ZAMS.L | 10.9 | 0.7        | 152.7737366 | -4.7030582 | 21.56  | 22.135 | 0.04            | 0.035           | -0.648 | -4.454 | 0.21           | 0.1  | 4.48      | 4.47      | 1.9            | 0.07              | 0.22              |
| 221 | TAMS.R | 10.9 | 1          | 152.7418663 | -4.6804666 | 20.231 | 20.664 | 0.03            | 0.016           | -0.506 | -5.783 | 1.84           | 21   | 4.38      | 3.65      | 5.3            | 0.04              | 0.14              |
| 222 | MS     | 10.9 | 0.5        | 152.7408534 | -4.7069695 | 20.446 | 20.955 | 0.021           | 0.018           | -0.582 | -5.568 | -              | 19.5 | 4.4       | 3.81      | 2.7            | 0.03              | 0.09              |
| 223 | MS     | 10.8 | 0.5        | 152.7227413 | -4.681354  | 21.568 | 22.134 | 0.03            | 0.022           | -0.639 | -4.446 | -              | 0.1  | 4.48      | 4.47      | 1.5            | 0.06              | 0.17              |
| 224 | MS     | 10.8 | 0.7        | 152.7706678 | -4.6996586 | 20.708 | 21.24  | 0.023           | 0.021           | -0.605 | -5.306 | -              | 17.2 | 4.43      | 3.99      | 3.8            | 0.03              | 0.11              |
| 225 | MS     | 10.8 | 0.9        | 152.7205744 | -4.689819  | 20.986 | 21.535 | 0.021           | 0.016           | -0.622 | -5.028 | -              | 13.4 | 4.45      | 4.17      | 5.1            | 0.03              | 0.12              |
| 226 | MS     | 10.8 | 0.5        | 152.7555773 | -4.6745795 | 20.41  | 20.912 | 0.021           | 0.022           | -0.575 | -5.604 | -              | 20.1 | 4.4       | 3.77      | 2.7            | 0.03              | 0.1               |
| 227 | MS     | 10.8 | 1.2        | 152.7520109 | -4.6682839 | 20.76  | 21.294 | 0.04            | 0.031           | -0.607 | -5.254 | -              | 16.9 | 4.44      | 4.02      | 7.1            | 0.05              | 0.19              |
| 228 | MS     | 10.7 | 0.9        | 152.7708514 | -4.7044874 | 20.719 | 21.249 | 0.029           | 0.022           | -0.603 | -5.295 | -              | 17.6 | 4.43      | 3.99      | 5              | 0.04              | 0.14              |
| 229 | MS     | 10.7 | 1.2        | 152.7547608 | -4.6971495 | 21.08  | 21.631 | 0.026           | 0.024           | -0.624 | -4.934 | -              | 12.3 | 4.46      | 4.21      | 7.7            | 0.04              | 0.15              |
| 230 | MS     | 10.7 | 0.7        | 152.7276739 | -4.6883876 | 20.862 | 21.401 | 0.02            | 0.018           | -0.612 | -5.152 | -              | 16   | 4.44      | 4.08      | 4.1            | 0.03              | 0.1               |
| 231 | MS     | 10.7 | 1.4        | 152.7691706 | -4.705387  | 20.953 | 21.497 | 0.038           | 0.036           | -0.617 | -5.061 | -              | 14.8 | 4.45      | 4.13      | 8.5            | 0.05              | 0.2               |
| 232 | MS     | 10.7 | 1.5        | 152.7557997 | -4.6963941 | 21.57  | 22.131 | 0.03            | 0.024           | -0.634 | -4.444 | -              | 1.1  | 4.47      | 4.44      | 10.7           | 0.05              | 0.2               |
| 233 | MS     | 10.7 | 1.2        | 152.7290134 | -4.6861724 | 21.178 | 21.731 | 0.024           | 0.017           | -0.626 | -4.836 | -              | 11   | 4.46      | 4.25      | 8.3            | 0.04              | 0.14              |
| 234 | ZAMS.L | 10.7 | 0.5        | 152.7691559 | -4.7054517 | 21.614 | 22.187 | 0.026           | 0.035           | -0.646 | -4.4   | 0.23           | 0.1  | 4.48      | 4.47      | 1.7            | 0.06              | 0.2               |
| 235 | MS     | 10.7 | 0.5        | 152.7714929 | -4.6968291 | 21.606 | 22.169 | 0.03            | 0.018           | -0.636 | -4.408 | -              | 0.2  | 4.48      | 4.46      | 1.4            | 0.05              | 0.16              |
| 236 | MS     | 10.7 | 3.4        | 152.7535715 | -4.6875776 | 21.53  | 22.09  | 0.046           | 0.034           | -0.633 | -4.484 | -              | 2.4  | 4.47      | 4.42      | 21.5           | 0.08              | 0.34              |
| 237 | MS     | 10.7 | 1          | 152.7571642 | -4.6906743 | 20.952 | 21.495 | 0.027           | 0.028           | -0.616 | -5.062 | -              | 15   | 4.45      | 4.12      | 6.3            | 0.04              | 0.15              |
| 238 | MS     | 10.7 | 0.7        | 152.7528663 | -4.6758246 | 20.72  | 21.247 | 0.023           | 0.023           | -0.6   | -5.294 | -              | 18   | 4.43      | 3.97      | 3.8            | 0.03              | 0.11              |
| 239 | MS     | 10.6 | 0.7        | 152.7212776 | -4.6928851 | 20.788 | 21.32  | 0.022           | 0.015           | -0.605 | -5.226 | -              | 17.3 | 4.43      | 4.02      | 3.9            | 0.03              | 0.1               |
| 240 | MS     | 10.6 | 0.7        | 152.7372188 | -4.6836991 | 20.351 | 20.841 | 0.024           | 0.017           | -0.563 | -5.663 | -              | 21.2 | 4.38      | 3.69      | 3.4            | 0.03              | 0.11              |
| 241 | MS     | 10.6 | 0.9        | 152.7282247 | -4.6932924 | 21.152 | 21.703 | 0.018           | 0.02            | -0.624 | -4.862 | -              | 11.8 | 4.46      | 4.23      | 6.3            | 0.03              | 0.12              |
| 242 | MS     | 10.6 | 0.5        | 152.7414321 | -4.7069477 | 20.546 | 21.055 | 0.02            | 0.019           | -0.582 | -5.468 | -              | 19.9 | 4.4       | 3.84      | 2.6            | 0.02              | 0.09              |
| 243 | TAMS.R | 10.6 | 0.8        | 152.7319568 | -4.6821321 | 20.306 | 20.754 | 0.021           | 0.021           | -0.521 | -5.708 | 1.77           | 21.8 | 4.38      | 3.66      | 4.2            | 0.03              | 0.11              |
| 244 | MS     | 10.6 | 1          | 152.7685553 | -4.7042708 | 20.981 | 21.524 | 0.027           | 0.024           | -0.616 | -5.033 | -              | 14.9 | 4.45      | 4.13      | 5.9            | 0.04              | 0.14              |
| 245 | ZAMS.L | 10.6 | 0.5        | 152.7295571 | -4.7030975 | 21.633 | 22.203 | 0.029           | 0.025           | -0.643 | -4.381 | 0.2            | 0.1  | 4.48      | 4.47      | 1.2            | 0.05              | 0.15              |

| IDN | Zone   | M    | $\sigma_M$ | RA          | Dec        | F275   | F336   | $\sigma_{F275}$ | $\sigma_{F336}$ | x      | y      | $d_x/\sigma_x$ | Age  | log(T) | log(g) | $\sigma_{Age}$ | $\sigma_{logT}$ | $\sigma_{logg}$ |
|-----|--------|------|------------|-------------|------------|--------|--------|-----------------|-----------------|--------|--------|----------------|------|--------|--------|----------------|-----------------|-----------------|
| 246 | MS     | 10.6 | 1.2        | 152.7244295 | -4.6991226 | 21.197 | 21.749 | 0.023           | 0.024           | -0.625 | -4.817 | -              | 11.1 | 4.46   | 4.25   | 8.2            | 0.03            | 0.15            |
| 247 | MS     | 10.6 | 0.9        | 152.74819   | -4.6717379 | 20.957 | 21.498 | 0.023           | 0.016           | -0.614 | -5.057 | -              | 15.4 | 4.44   | 4.11   | 5.1            | 0.03            | 0.12            |
| 248 | MS     | 10.6 | 1          | 152.7430804 | -4.6787616 | 21.108 | 21.656 | 0.016           | 0.025           | -0.621 | -4.906 | -              | 13.1 | 4.45   | 4.2    | 6.7            | 0.03            | 0.14            |
| 249 | MS     | 10.6 | 1.6        | 152.7269024 | -4.6854166 | 21.487 | 22.045 | 0.019           | 0.025           | -0.631 | -4.527 | -              | 4.5  | 4.47   | 4.39   | 13             | 0.04            | 0.18            |
| 250 | MS     | 10.6 | 1.3        | 152.7318754 | -4.7153222 | 21.045 | 21.59  | 0.033           | 0.031           | -0.618 | -4.969 | -              | 14.2 | 4.45   | 4.16   | 8.3            | 0.04            | 0.17            |
| 251 | MS     | 10.5 | 1          | 152.7412359 | -4.670107  | 20.882 | 21.417 | 0.021           | 0.032           | -0.608 | -5.132 | -              | 16.8 | 4.44   | 4.06   | 6.2            | 0.04            | 0.17            |
| 252 | MS     | 10.5 | 0.6        | 152.7523896 | -4.6784212 | 20.582 | 21.091 | 0.023           | 0.015           | -0.582 | -5.432 | -              | 20.1 | 4.4    | 3.85   | 3.1            | 0.03            | 0.1             |
| 253 | MS     | 10.5 | 1.8        | 152.7249849 | -4.6885646 | 21.53  | 22.088 | 0.027           | 0.019           | -0.631 | -4.484 | -              | 3.6  | 4.47   | 4.4    | 13.5           | 0.04            | 0.18            |
| 254 | MS     | 10.5 | 0.9        | 152.7409525 | -4.6704969 | 20.829 | 21.36  | 0.03            | 0.02            | -0.604 | -5.185 | -              | 17.5 | 4.43   | 4.02   | 5.2            | 0.04            | 0.14            |
| 255 | MS     | 10.5 | 1.6        | 152.7580197 | -4.7013415 | 21.408 | 21.964 | 0.019           | 0.027           | -0.629 | -4.606 | -              | 6.9  | 4.46   | 4.35   | 11.6           | 0.04            | 0.18            |
| 256 | MS     | 10.5 | 1.6        | 152.754003  | -4.6819821 | 21.277 | 21.83  | 0.03            | 0.015           | -0.626 | -4.737 | -              | 9.9  | 4.46   | 4.28   | 10.6           | 0.04            | 0.18            |
| 257 | MS     | 10.5 | 1.7        | 152.7566427 | -4.6756555 | 21.361 | 21.916 | 0.03            | 0.028           | -0.628 | -4.653 | -              | 8.1  | 4.46   | 4.32   | 12.7           | 0.05            | 0.19            |
| 258 | ZAMS_L | 10.5 | 0.4        | 152.733961  | -4.6763657 | 21.652 | 22.266 | 0.024           | 0.027           | -0.687 | -4.362 | 1.88           | 0.1  | 4.48   | 4.47   | 1.2            | 0.04            | 0.14            |
| 259 | ZAMS_L | 10.5 | 0.5        | 152.7222971 | -4.6958158 | 21.653 | 22.226 | 0.034           | 0.021           | -0.646 | -4.361 | 0.29           | 0.1  | 4.48   | 4.47   | 1.5            | 0.06            | 0.17            |
| 260 | MS     | 10.5 | 1.8        | 152.7412638 | -4.6749785 | 21.369 | 21.924 | 0.029           | 0.032           | -0.628 | -4.645 | -              | 8    | 4.46   | 4.33   | 13.7           | 0.05            | 0.22            |
| 261 | MS     | 10.5 | 2          | 152.7598602 | -4.6825167 | 21.64  | 22.2   | 0.038           | 0.035           | -0.633 | -4.374 | -              | 0.4  | 4.47   | 4.45   | 13.7           | 0.06            | 0.25            |
| 262 | MS     | 10.5 | 1.5        | 152.7528055 | -4.693291  | 21.612 | 22.171 | 0.028           | 0.026           | -0.632 | -4.402 | -              | 1.2  | 4.47   | 4.44   | 10.1           | 0.05            | 0.18            |
| 263 | ZAMS_L | 10.5 | 0.5        | 152.744575  | -4.6756526 | 21.661 | 22.234 | 0.03            | 0.021           | -0.646 | -4.353 | 0.33           | 0.1  | 4.48   | 4.47   | 1.3            | 0.05            | 0.15            |
| 264 | TAMS_R | 10.5 | 0.7        | 152.7697121 | -4.7026925 | 20.339 | 20.79  | 0.02            | 0.015           | -0.524 | -5.675 | 1.62           | 22.2 | 4.37   | 3.66   | 4              | 0.02            | 0.1             |
| 265 | MS     | 10.5 | 0.8        | 152.7377243 | -4.6765574 | 20.977 | 21.516 | 0.02            | 0.024           | -0.612 | -5.037 | -              | 15.8 | 4.44   | 4.11   | 5.2            | 0.03            | 0.13            |
| 266 | MS     | 10.5 | 1.1        | 152.7381154 | -4.6774285 | 21.143 | 21.69  | 0.025           | 0.025           | -0.62  | -4.871 | -              | 13.1 | 4.45   | 4.21   | 7.6            | 0.03            | 0.14            |
| 267 | MS     | 10.5 | 1.4        | 152.7269896 | -4.6887416 | 21.414 | 21.969 | 0.024           | 0.023           | -0.628 | -4.6   | -              | 7.3  | 4.46   | 4.34   | 10.5           | 0.04            | 0.15            |
| 268 | MS     | 10.4 | 0.5        | 152.7471781 | -4.6752228 | 20.642 | 21.153 | 0.017           | 0.018           | -0.584 | -5.372 | -              | 20.1 | 4.41   | 3.87   | 2.4            | 0.02            | 0.08            |
| 269 | MS     | 10.4 | 1.6        | 152.7586501 | -4.684388  | 21.247 | 21.797 | 0.032           | 0.035           | -0.623 | -4.767 | -              | 11.3 | 4.46   | 4.26   | 12.4           | 0.05            | 0.21            |
| 270 | ZAMS_L | 10.4 | 0.6        | 152.7525543 | -4.6819877 | 21.678 | 22.29  | 0.039           | 0.024           | -0.685 | -4.336 | 1.27           | 0.1  | 4.47   | 4.48   | 1.7            | 0.06            | 0.2             |
| 271 | MS     | 10.4 | 0.7        | 152.7414588 | -4.679354  | 21.03  | 21.57  | 0.016           | 0.021           | -0.613 | -4.984 | -              | 15.5 | 4.44   | 4.13   | 4.8            | 0.03            | 0.11            |
| 272 | ZAMS_L | 10.4 | 0.4        | 152.7618255 | -4.7006865 | 21.686 | 22.257 | 0.026           | 0.031           | -0.644 | -4.328 | 0.29           | 0.1  | 4.47   | 4.48   | 1.4            | 0.05            | 0.16            |
| 273 | ZAMS_L | 10.4 | 0.7        | 152.7337024 | -4.6732995 | 21.687 | 22.327 | 0.044           | 0.029           | -0.713 | -4.327 | 1.77           | 0.1  | 4.47   | 4.48   | 1.9            | 0.07            | 0.22            |
| 274 | MS     | 10.4 | 1.9        | 152.7210455 | -4.6903572 | 21.475 | 22.03  | 0.031           | 0.027           | -0.628 | -4.539 | -              | 6.2  | 4.46   | 4.36   | 15             | 0.05            | 0.2             |
| 275 | MS     | 10.4 | 0.6        | 152.7408017 | -4.677318  | 20.671 | 21.182 | 0.021           | 0.017           | -0.584 | -5.343 | -              | 20.2 | 4.41   | 3.88   | 3              | 0.03            | 0.09            |
| 276 | ZAMS_L | 10.4 | 0.7        | 152.7414169 | -4.6941432 | 21.698 | 22.321 | 0.045           | 0.038           | -0.696 | -4.316 | 1.37           | 0.1  | 4.47   | 4.48   | 1.9            | 0.07            | 0.23            |
| 277 | TAMS_R | 10.3 | 0.9        | 152.7443942 | -4.7121531 | 20.376 | 20.843 | 0.025           | 0.023           | -0.54  | -5.638 | 0.59           | 22.7 | 4.37   | 3.66   | 4.9            | 0.03            | 0.12            |
| 278 | ZAMS_L | 10.3 | 0.4        | 152.7680315 | -4.7020366 | 21.705 | 22.284 | 0.028           | 0.02            | -0.652 | -4.309 | 0.63           | 0.1  | 4.47   | 4.48   | 1.1            | 0.04            | 0.13            |
| 279 | MS     | 10.3 | 0.7        | 152.7677296 | -4.7052832 | 20.959 | 21.492 | 0.014           | 0.022           | -0.606 | -5.055 | -              | 17.1 | 4.43   | 4.07   | 4.3            | 0.03            | 0.11            |
| 280 | MS     | 10.3 | 0.5        | 152.74003   | -4.6758279 | 21.71  | 22.271 | 0.031           | 0.019           | -0.634 | -4.304 | -              | 0.1  | 4.47   | 4.48   | 1.3            | 0.05            | 0.16            |
| 281 | MS     | 10.3 | 0.8        | 152.7241373 | -4.6878867 | 20.449 | 20.934 | 0.021           | 0.032           | -0.558 | -5.565 | -              | 22.4 | 4.38   | 3.7    | 4.4            | 0.04            | 0.15            |
| 282 | ZAMS_L | 10.3 | 0.4        | 152.7575293 | -4.7085751 | 21.716 | 22.286 | 0.028           | 0.021           | -0.643 | -4.298 | 0.33           | 0.1  | 4.47   | 4.48   | 1.1            | 0.04            | 0.13            |
| 283 | MS     | 10.3 | 1.8        | 152.7197928 | -4.6974101 | 21.441 | 21.993 | 0.033           | 0.027           | -0.625 | -4.573 | -              | 8.2  | 4.46   | 4.33   | 14             | 0.05            | 0.2             |
| 284 | MS     | 10.3 | 0.7        | 152.7239003 | -4.6993925 | 20.75  | 21.264 | 0.024           | 0.023           | -0.587 | -5.264 | -              | 20.1 | 4.41   | 3.92   | 3.5            | 0.03            | 0.11            |
| 285 | MS     | 10.3 | 0.9        | 152.7386282 | -4.6755979 | 21.13  | 21.671 | 0.024           | 0.017           | -0.614 | -4.884 | -              | 14.8 | 4.44   | 4.17   | 6.1            | 0.03            | 0.12            |
| 286 | MS     | 10.2 | 0.5        | 152.7234401 | -4.6870222 | 20.548 | 21.041 | 0.02            | 0.018           | -0.566 | -5.466 | -              | 22   | 4.39   | 3.76   | 2.6            | 0.02            | 0.09            |
| 287 | MS     | 10.2 | 1.5        | 152.7520679 | -4.6932835 | 21.298 | 21.845 | 0.031           | 0.026           | -0.62  | -4.716 | -              | 11.9 | 4.45   | 4.25   | 10.4           | 0.04            | 0.17            |
| 288 | MS     | 10.2 | 1.7        | 152.7241816 | -4.6965382 | 21.48  | 22.032 | 0.03            | 0.022           | -0.625 | -4.534 | -              | 7.5  | 4.46   | 4.34   | 12.4           | 0.04            | 0.18            |
| 289 | MS     | 10.2 | 2.1        | 152.7494778 | -4.672584  | 21.584 | 22.138 | 0.033           | 0.026           | -0.627 | -4.43  | -              | 4.6  | 4.46   | 4.39   | 16.5           | 0.05            | 0.21            |
| 290 | ZAMS_L | 10.2 | 0.6        | 152.7461925 | -4.7058518 | 21.737 | 22.302 | 0.043           | 0.037           | -0.638 | -4.277 | 0.12           | 0.1  | 4.47   | 4.48   | 1.7            | 0.07            | 0.21            |

| IDN | Zone   | M    | $\sigma_M$ | RA          | Dec        | F275   | F336   | $\sigma_{F275}$ | $\sigma_{F336}$ | x      | y      | $d_x/\sigma_x$ | Age  | log(T) | log(g) | $\sigma_{Age}$ | $\sigma_{logT}$ | $\sigma_{logg}$ |
|-----|--------|------|------------|-------------|------------|--------|--------|-----------------|-----------------|--------|--------|----------------|------|--------|--------|----------------|-----------------|-----------------|
| 291 | MS     | 10.2 | 2.3        | 152.7514201 | -4.6784868 | 21.508 | 22.06  | 0.041           | 0.024           | -0.625 | -4.506 | -              | 7.1  | 4.46   | 4.35   | 17.5           | 0.06            | 0.25            |
| 292 | ZAMS L | 10.2 | 0.5        | 152.7270935 | -4.6878437 | 21.746 | 22.364 | 0.031           | 0.031           | -0.691 | -4.268 | 1.88           | 0.1  | 4.47   | 4.48   | 1.3            | 0.05            | 0.16            |
| 293 | MS     | 10.1 | 0.6        | 152.7441677 | -4.7039749 | 20.81  | 21.325 | 0.02            | 0.019           | -0.588 | -5.204 | -              | 20.1 | 4.41   | 3.94   | 3              | 0.02            | 0.09            |
| 294 | MS     | 10.1 | 0.9        | 152.737112  | -4.6757847 | 20.934 | 21.459 | 0.022           | 0.032           | -0.598 | -5.08  | -              | 18.6 | 4.42   | 4.03   | 5.9            | 0.04            | 0.16            |
| 295 | MS     | 10.1 | 0.7        | 152.7695053 | -4.6985212 | 20.871 | 21.391 | 0.025           | 0.022           | -0.593 | -5.143 | -              | 19.4 | 4.42   | 3.98   | 4.3            | 0.03            | 0.11            |
| 296 | MS     | 10.1 | 0.5        | 152.7287249 | -4.6774432 | 21.755 | 22.313 | 0.035           | 0.035           | -0.631 | -4.259 | -              | 0.2  | 4.47   | 4.47   | 1.5            | 0.05            | 0.18            |
| 297 | MS     | 10.1 | 1.7        | 152.7625459 | -4.7073857 | 21.697 | 22.251 | 0.025           | 0.019           | -0.627 | -4.317 | -              | 1.8  | 4.46   | 4.43   | 14.7           | 0.04            | 0.17            |
| 298 | MS     | 10.1 | 0.5        | 152.7449422 | -4.6757217 | 20.661 | 21.161 | 0.021           | 0.015           | -0.573 | -5.353 | -              | 21.6 | 4.39   | 3.83   | 2.8            | 0.03            | 0.09            |
| 299 | MS     | 10.1 | 1.1        | 152.7221869 | -4.7022662 | 20.968 | 21.495 | 0.034           | 0.027           | -0.6   | -5.046 | -              | 18.3 | 4.43   | 4.05   | 6.6            | 0.04            | 0.16            |
| 300 | MS     | 10.1 | 0.6        | 152.7276374 | -4.6812055 | 20.782 | 21.292 | 0.021           | 0.021           | -0.583 | -5.232 | -              | 20.8 | 4.41   | 3.91   | 3.1            | 0.03            | 0.1             |
| 301 | MS     | 10.1 | 2.1        | 152.769116  | -4.7055095 | 21.344 | 21.889 | 0.037           | 0.042           | -0.618 | -4.67  | -              | 12.1 | 4.45   | 4.26   | 19.7           | 0.06            | 0.26            |
| 302 | TAMS R | 10   | 2.2        | 152.7228228 | -4.6866972 | 20.462 | 20.938 | 0.037           | 0.042           | -0.549 | -5.552 | 0.04           | 23.8 | 4.37   | 3.67   | 17.5           | 0.05            | 0.25            |
| 303 | MS     | 10   | 0.7        | 152.7411963 | -4.6770842 | 20.588 | 21.076 | 0.023           | 0.025           | -0.561 | -5.426 | -              | 22.9 | 4.38   | 3.75   | 5.1            | 0.03            | 0.12            |
| 304 | MS     | 10   | 1.3        | 152.7561494 | -4.6811079 | 21.263 | 21.804 | 0.029           | 0.022           | -0.614 | -4.751 | -              | 14.1 | 4.44   | 4.21   | 11.1           | 0.04            | 0.16            |
| 305 | MS     | 10   | 1.1        | 152.7382119 | -4.6837659 | 21.13  | 21.664 | 0.027           | 0.022           | -0.607 | -4.884 | -              | 16.7 | 4.43   | 4.13   | 9.2            | 0.03            | 0.14            |
| 306 | MS     | 10   | 0.8        | 152.7426581 | -4.6793779 | 20.879 | 21.395 | 0.025           | 0.021           | -0.589 | -5.135 | -              | 20.2 | 4.41   | 3.97   | 6.4            | 0.03            | 0.12            |
| 307 | MS     | 10   | 0.8        | 152.7712212 | -4.7025736 | 20.899 | 21.416 | 0.025           | 0.014           | -0.59  | -5.115 | -              | 20.2 | 4.41   | 3.98   | 6.3            | 0.03            | 0.12            |
| 308 | ZAMS L | 10   | 0.4        | 152.726506  | -4.688088  | 21.797 | 22.398 | 0.031           | 0.018           | -0.674 | -4.217 | 1.41           | 0.1  | 4.47   | 4.48   | 1.2            | 0.05            | 0.14            |
| 309 | ZAMS L | 10   | 0.5        | 152.7493108 | -4.6738249 | 21.805 | 22.418 | 0.041           | 0.03            | -0.686 | -4.209 | 1.36           | 0.1  | 4.47   | 4.48   | 1.5            | 0.06            | 0.18            |
| 310 | ZAMS L | 10   | 0.4        | 152.7263607 | -4.6865822 | 21.806 | 22.367 | 0.033           | 0.028           | -0.634 | -4.208 | 0.12           | 0.1  | 4.47   | 4.48   | 1.2            | 0.05            | 0.15            |
| 311 | MS     | 9.9  | 1.6        | 152.7567876 | -4.6839136 | 21.16  | 21.694 | 0.04            | 0.022           | -0.607 | -4.854 | -              | 16.7 | 4.43   | 4.14   | 13.4           | 0.05            | 0.21            |
| 312 | MS     | 9.9  | 0.9        | 152.7242032 | -4.7026159 | 20.6   | 21.086 | 0.032           | 0.024           | -0.559 | -5.414 | -              | 23.5 | 4.38   | 3.75   | 7              | 0.04            | 0.15            |
| 313 | MS     | 9.9  | 2.1        | 152.7246194 | -4.6953107 | 21.488 | 22.035 | 0.038           | 0.021           | -0.62  | -4.526 | -              | 9.8  | 4.45   | 4.32   | 18.6           | 0.05            | 0.23            |
| 314 | MS     | 9.9  | 1.6        | 152.7328439 | -4.6872982 | 21.466 | 22.012 | 0.03            | 0.022           | -0.619 | -4.548 | -              | 10.6 | 4.45   | 4.3    | 14.1           | 0.04            | 0.18            |
| 315 | MS     | 9.9  | 1.1        | 152.7478933 | -4.6733289 | 21.809 | 22.362 | 0.036           | 0.022           | -0.626 | -4.205 | -              | 0.4  | 4.46   | 4.46   | 8.5            | 0.05            | 0.19            |
| 316 | MS     | 9.9  | 1.7        | 152.7549234 | -4.6911854 | 21.379 | 21.922 | 0.036           | 0.025           | -0.616 | -4.635 | -              | 12.7 | 4.45   | 4.26   | 15.2           | 0.05            | 0.21            |
| 317 | MS     | 9.9  | 0.5        | 152.7478664 | -4.7087275 | 20.721 | 21.218 | 0.018           | 0.018           | -0.57  | -5.293 | -              | 22.8 | 4.39   | 3.83   | 4.1            | 0.02            | 0.09            |
| 318 | MS     | 9.9  | 1          | 152.7476194 | -4.7061787 | 20.555 | 21.034 | 0.03            | 0.023           | -0.552 | -5.459 | -              | 24.4 | 4.37   | 3.7    | 7.8            | 0.04            | 0.14            |
| 319 | TAMS R | 9.8  | 1.3        | 152.7455106 | -4.6810459 | 20.519 | 20.976 | 0.024           | 0.02            | -0.53  | -5.495 | 0.83           | 24.8 | 4.37   | 3.68   | 10.3           | 0.03            | 0.14            |
| 320 | TAMS R | 9.8  | 1.2        | 152.7336271 | -4.7119829 | 20.519 | 20.983 | 0.022           | 0.017           | -0.537 | -5.495 | 0.58           | 24.8 | 4.37   | 3.68   | 9.4            | 0.03            | 0.12            |
| 321 | MS     | 9.8  | 0.9        | 152.7485747 | -4.6784229 | 21.102 | 21.63  | 0.023           | 0.025           | -0.601 | -4.912 | -              | 18.5 | 4.43   | 4.09   | 7.8            | 0.03            | 0.13            |
| 322 | TAMS R | 9.8  | 1.3        | 152.7469295 | -4.7159445 | 20.522 | 20.959 | 0.025           | 0.023           | -0.51  | -5.492 | 1.59           | 24.9 | 4.37   | 3.68   | 10.7           | 0.03            | 0.14            |
| 323 | MS     | 9.8  | 0.6        | 152.7659067 | -4.7056769 | 21.041 | 21.564 | 0.016           | 0.02            | -0.596 | -4.973 | -              | 19.7 | 4.42   | 4.05   | 5.7            | 0.02            | 0.1             |
| 324 | ZAMS L | 9.8  | 0.5        | 152.7250927 | -4.6951662 | 21.849 | 22.422 | 0.042           | 0.034           | -0.646 | -4.165 | 0.43           | 0.1  | 4.46   | 4.48   | 1.6            | 0.06            | 0.19            |
| 325 | MS     | 9.8  | 0.6        | 152.769468  | -4.704238  | 20.929 | 21.442 | 0.02            | 0.015           | -0.586 | -5.085 | -              | 21.4 | 4.41   | 3.96   | 5.2            | 0.02            | 0.09            |
| 326 | MS     | 9.8  | 1.9        | 152.7447153 | -4.715735  | 21.269 | 21.805 | 0.045           | 0.035           | -0.609 | -4.745 | -              | 16.1 | 4.44   | 4.18   | 18             | 0.06            | 0.24            |
| 327 | MS     | 9.8  | 1.4        | 152.754889  | -4.6805904 | 21.278 | 21.814 | 0.033           | 0.027           | -0.609 | -4.736 | -              | 16.1 | 4.44   | 4.18   | 13.2           | 0.04            | 0.18            |
| 328 | TAMS R | 9.8  | 0.9        | 152.7284554 | -4.7083587 | 20.547 | 20.999 | 0.017           | 0.02            | -0.525 | -5.467 | 1.22           | 25.3 | 4.37   | 3.68   | 7.7            | 0.02            | 0.11            |
| 329 | MS     | 9.7  | 1.2        | 152.7639965 | -4.7023841 | 21.295 | 21.831 | 0.028           | 0.022           | -0.609 | -4.719 | -              | 16.1 | 4.44   | 4.19   | 11.5           | 0.04            | 0.15            |
| 330 | MS     | 9.7  | 1.3        | 152.7199035 | -4.6961207 | 21.348 | 21.886 | 0.028           | 0.025           | -0.611 | -4.666 | -              | 15.1 | 4.44   | 4.22   | 12             | 0.04            | 0.15            |
| 331 | MS     | 9.7  | 1          | 152.737977  | -4.6740883 | 21.017 | 21.535 | 0.03            | 0.022           | -0.591 | -4.997 | -              | 20.9 | 4.42   | 4.01   | 8.8            | 0.04            | 0.15            |
| 332 | MS     | 9.7  | 0.8        | 152.7383881 | -4.6708059 | 21.058 | 21.579 | 0.023           | 0.02            | -0.594 | -4.956 | -              | 20.4 | 4.42   | 4.04   | 7.3            | 0.03            | 0.12            |
| 333 | ZAMS L | 9.7  | 0.4        | 152.7194902 | -4.6944561 | 21.878 | 22.46  | 0.04            | 0.024           | -0.655 | -4.136 | 0.7            | 0.1  | 4.46   | 4.48   | 1.4            | 0.06            | 0.17            |
| 334 | MS     | 9.7  | 1.9        | 152.7682186 | -4.6972072 | 21.697 | 22.244 | 0.024           | 0.033           | -0.62  | -4.317 | -              | 6.2  | 4.45   | 4.38   | 19.8           | 0.05            | 0.22            |
| 335 | MS     | 9.7  | 1          | 152.7365417 | -4.703917  | 20.711 | 21.2   | 0.032           | 0.021           | -0.562 | -5.303 | -              | 24.4 | 4.38   | 3.79   | 7.7            | 0.04            | 0.15            |



| IDN | Zone   | M   | $\sigma_M$ | RA          | Dec        | F275   | F336   | $\sigma_{F275}$ | $\sigma_{F336}$ | x      | y      | $d_n/\sigma_x$ | Age  | log(T) | log(g) | $\sigma_{Age}$ | $\sigma_{logT}$ | $\sigma_{logg}$ |
|-----|--------|-----|------------|-------------|------------|--------|--------|-----------------|-----------------|--------|--------|----------------|------|--------|--------|----------------|-----------------|-----------------|
| 336 | TAMS.R | 9.7 | 1.2        | 152.7690797 | -4.6973476 | 20.563 | 21.103 | 0.025           | 0.021           | -0.54  | -5.451 | 0.37           | 25.6 | 4.36   | 3.69   | 9.9            | 0.03            | 0.13            |
| 337 | MS     | 9.7 | 1.3        | 152.7385377 | -4.6719391 | 21.585 | 22.13  | 0.023           | 0.02            | -0.618 | -4.429 | -              | 9.6  | 4.45   | 4.33   | 12.5           | 0.03            | 0.14            |
| 338 | TAMS.R | 9.7 | 1.5        | 152.7415612 | -4.6785992 | 20.568 | 21.036 | 0.031           | 0.019           | -0.541 | -5.446 | 0.26           | 25.7 | 4.36   | 3.69   | 12.3           | 0.04            | 0.17            |
| 339 | MS     | 9.7 | 0.8        | 152.7698986 | -4.7048066 | 21.031 | 21.549 | 0.024           | 0.024           | -0.591 | -4.983 | -              | 21.1 | 4.42   | 4.02   | 7.4            | 0.03            | 0.13            |
| 340 | ZAMS.L | 9.7 | 0.3        | 152.7450436 | -4.7132293 | 21.886 | 22.456 | 0.031           | 0.029           | -0.643 | -4.128 | 0.53           | 0.1  | 4.46   | 4.48   | 1.1            | 0.04            | 0.13            |
| 341 | MS     | 9.7 | 1          | 152.7204931 | -4.6935648 | 21.074 | 21.595 | 0.029           | 0.028           | -0.594 | -4.94  | -              | 20.5 | 4.42   | 4.04   | 9.2            | 0.04            | 0.15            |
| 342 | MS     | 9.7 | 0.9        | 152.7261941 | -4.6863461 | 21.037 | 21.555 | 0.025           | 0.028           | -0.591 | -4.977 | -              | 21.1 | 4.42   | 4.02   | 8.3            | 0.03            | 0.15            |
| 343 | MS     | 9.7 | 2.4        | 152.7238789 | -4.6980148 | 21.837 | 22.385 | 0.042           | 0.032           | -0.621 | -4.177 | -              | 1.6  | 4.45   | 4.44   | 25.4           | 0.06            | 0.26            |
| 344 | ZAMS.L | 9.6 | 0.3        | 152.7407757 | -4.7184277 | 21.9   | 22.456 | 0.029           | 0.023           | -0.629 | -4.114 | 0.11           | 0.1  | 4.46   | 4.48   | 1              | 0.04            | 0.12            |
| 345 | ZAMS.L | 9.6 | 0.2        | 152.77015   | -4.7045198 | 21.906 | 22.46  | 0.025           | 0.024           | -0.627 | -4.108 | 0.06           | 0.1  | 4.46   | 4.48   | 0.9            | 0.04            | 0.11            |
| 346 | MS     | 9.6 | 1.3        | 152.7268715 | -4.681444  | 21.474 | 22.014 | 0.027           | 0.028           | -0.613 | -4.54  | -              | 13.6 | 4.44   | 4.27   | 14.3           | 0.04            | 0.17            |
| 347 | MS     | 9.6 | 0.8        | 152.7376958 | -4.7143494 | 20.919 | 21.424 | 0.025           | 0.015           | -0.578 | -5.095 | -              | 23.4 | 4.4    | 3.92   | 6.8            | 0.03            | 0.12            |
| 348 | MS     | 9.6 | 0.9        | 152.7375196 | -4.6752159 | 20.897 | 21.4   | 0.028           | 0.031           | -0.576 | -5.117 | -              | 23.6 | 4.4    | 3.91   | 7.9            | 0.04            | 0.15            |
| 349 | MS     | 9.6 | 0.9        | 152.7715318 | -4.703201  | 21.284 | 21.815 | 0.017           | 0.023           | -0.604 | -4.73  | -              | 18.1 | 4.43   | 4.16   | 9              | 0.03            | 0.13            |
| 350 | TAMS.R | 9.6 | 1.4        | 152.7483333 | -4.7160553 | 20.612 | 21.028 | 0.031           | 0.022           | -0.489 | -5.402 | 1.92           | 26.5 | 4.36   | 3.7    | 12.3           | 0.04            | 0.17            |
| 351 | MS     | 9.6 | 0.7        | 152.737463  | -4.6752548 | 20.95  | 21.457 | 0.022           | 0.022           | -0.58  | -5.064 | -              | 23.3 | 4.4    | 3.94   | 6.1            | 0.03            | 0.11            |
| 352 | MS     | 9.6 | 0.9        | 152.7405986 | -4.6889867 | 21.036 | 21.55  | 0.026           | 0.022           | -0.587 | -4.978 | -              | 22.3 | 4.41   | 4      | 7.7            | 0.03            | 0.13            |
| 353 | ZAMS.L | 9.6 | 0.4        | 152.7529092 | -4.6799823 | 21.925 | 22.514 | 0.046           | 0.041           | -0.662 | -4.089 | 0.81           | 0.1  | 4.46   | 4.48   | 1.6            | 0.06            | 0.19            |
| 354 | MS     | 9.5 | 0.3        | 152.7475813 | -4.6762906 | 21.927 | 22.477 | 0.033           | 0.029           | -0.623 | -4.087 | -              | 0.2  | 4.46   | 4.48   | 1.2            | 0.05            | 0.14            |
| 355 | MS     | 9.5 | 1.2        | 152.7291568 | -4.6985243 | 21.258 | 21.787 | 0.031           | 0.026           | -0.602 | -4.756 | -              | 18.8 | 4.43   | 4.14   | 11.7           | 0.04            | 0.16            |
| 356 | MS     | 9.5 | 0.6        | 152.7706767 | -4.7007409 | 20.93  | 21.434 | 0.018           | 0.015           | -0.577 | -5.084 | -              | 23.8 | 4.4    | 3.92   | 5              | 0.02            | 0.09            |
| 357 | MS     | 9.5 | 0.6        | 152.7677296 | -4.7053755 | 20.713 | 21.195 | 0.019           | 0.014           | -0.555 | -5.301 | -              | 26   | 4.37   | 3.76   | 4.7            | 0.02            | 0.09            |
| 358 | MS     | 9.5 | 0.9        | 152.7513994 | -4.6772217 | 21.054 | 21.568 | 0.024           | 0.029           | -0.587 | -4.96  | -              | 22.4 | 4.41   | 4      | 8.3            | 0.04            | 0.15            |
| 359 | TAMS.R | 9.5 | 1.2        | 152.7278131 | -4.6914484 | 20.627 | 21.101 | 0.025           | 0.02            | -0.547 | -5.387 | 0.05           | 26.8 | 4.36   | 3.7    | 9.9            | 0.03            | 0.13            |
| 360 | MS     | 9.5 | 0.2        | 152.7245859 | -4.6881987 | 21.938 | 22.488 | 0.025           | 0.025           | -0.623 | -4.076 | -              | 0.2  | 4.46   | 4.48   | 0.9            | 0.04            | 0.11            |
| 361 | MS     | 9.5 | 0.8        | 152.7264965 | -4.6959684 | 21.084 | 21.6   | 0.024           | 0.02            | -0.589 | -4.93  | -              | 22.1 | 4.41   | 4.02   | 7.3            | 0.03            | 0.12            |
| 362 | MS     | 9.5 | 1.9        | 152.7342157 | -4.7026769 | 21.581 | 22.122 | 0.027           | 0.035           | -0.614 | -4.433 | -              | 12   | 4.44   | 4.31   | 20.4           | 0.05            | 0.22            |
| 363 | ZAMS.L | 9.5 | 0.2        | 152.7549138 | -4.7060524 | 21.945 | 22.512 | 0.031           | 0.028           | -0.64  | -4.069 | 0.52           | 0.2  | 4.46   | 4.48   | 1              | 0.04            | 0.12            |
| 364 | MS     | 9.5 | 1.5        | 152.7459475 | -4.7103269 | 21.247 | 21.774 | 0.036           | 0.034           | -0.6   | -4.767 | -              | 19.5 | 4.43   | 4.13   | 13.7           | 0.04            | 0.19            |
| 365 | MS     | 9.5 | 1.4        | 152.7296686 | -4.687955  | 21.436 | 21.972 | 0.028           | 0.029           | -0.609 | -4.578 | -              | 15.8 | 4.44   | 4.23   | 14.3           | 0.04            | 0.17            |
| 366 | ZAMS.L | 9.5 | 0.4        | 152.7194171 | -4.6886705 | 21.946 | 22.516 | 0.048           | 0.026           | -0.643 | -4.068 | 0.4            | 0.2  | 4.46   | 4.48   | 1.6            | 0.07            | 0.19            |
| 367 | MS     | 9.5 | 1.3        | 152.7242876 | -4.6993361 | 21.254 | 21.781 | 0.032           | 0.028           | -0.6   | -4.76  | -              | 19.6 | 4.43   | 4.13   | 12.2           | 0.04            | 0.17            |
| 368 | MS     | 9.5 | 0.3        | 152.7281257 | -4.68464   | 21.946 | 22.494 | 0.031           | 0.032           | -0.621 | -4.068 | -              | 0.3  | 4.45   | 4.47   | 1.2            | 0.04            | 0.14            |
| 369 | ZAMS.L | 9.5 | 0.3        | 152.7496957 | -4.6835852 | 21.951 | 22.506 | 0.04            | 0.027           | -0.628 | -4.063 | 0.11           | 0.2  | 4.46   | 4.49   | 1.3            | 0.05            | 0.16            |
| 370 | MS     | 9.4 | 1.1        | 152.7308793 | -4.6887044 | 21.232 | 21.757 | 0.027           | 0.025           | -0.598 | -4.782 | -              | 20.2 | 4.42   | 4.11   | 9.9            | 0.03            | 0.14            |
| 371 | MS     | 9.4 | 0.8        | 152.7245275 | -4.699076  | 20.838 | 21.33  | 0.026           | 0.023           | -0.565 | -5.176 | -              | 25.5 | 4.38   | 3.84   | 6.5            | 0.03            | 0.12            |
| 372 | MS     | 9.4 | 1.5        | 152.7554207 | -4.7112859 | 20.653 | 21.128 | 0.016           | 0.035           | -0.548 | -5.361 | -              | 27.2 | 4.36   | 3.7    | 13.2           | 0.04            | 0.2             |
| 373 | MS     | 9.4 | 2          | 152.7505686 | -4.6704595 | 21.632 | 22.173 | 0.035           | 0.02            | -0.614 | -4.382 | -              | 11.4 | 4.44   | 4.32   | 21.1           | 0.05            | 0.21            |
| 374 | MS     | 9.4 | 2.6        | 152.7560465 | -4.6855555 | 21.784 | 22.327 | 0.042           | 0.034           | -0.616 | -4.23  | -              | 6.7  | 4.45   | 4.39   | 27.2           | 0.06            | 0.26            |
| 375 | TAMS.R | 9.4 | 1.1        | 152.7707449 | -4.700328  | 20.659 | 21.122 | 0.023           | 0.017           | -0.536 | -5.355 | 0.5            | 27.4 | 4.36   | 3.7    | 9.1            | 0.03            | 0.12            |
| 376 | TAMS.R | 9.4 | 0.9        | 152.7491245 | -4.6808081 | 20.662 | 21.127 | 0.02            | 0.018           | -0.538 | -5.352 | 0.47           | 27.5 | 4.36   | 3.7    | 7.9            | 0.02            | 0.11            |
| 377 | MS     | 9.4 | 1.6        | 152.7701271 | -4.7049002 | 21.397 | 21.929 | 0.036           | 0.031           | -0.605 | -4.617 | -              | 17.7 | 4.43   | 4.2    | 15.5           | 0.05            | 0.2             |
| 378 | MS     | 9.4 | 1.1        | 152.7341971 | -4.6736449 | 21.678 | 22.219 | 0.018           | 0.02            | -0.614 | -4.336 | -              | 10.7 | 4.44   | 4.34   | 11.9           | 0.03            | 0.13            |
| 379 | MS     | 9.4 | 0.9        | 152.7253473 | -4.6869598 | 21.1   | 21.613 | 0.023           | 0.029           | -0.586 | -4.914 | -              | 23.2 | 4.41   | 4.01   | 8.6            | 0.04            | 0.15            |
| 380 | ZAMS.L | 9.3 | 0.2        | 152.7249983 | -4.689612  | 21.987 | 22.55  | 0.033           | 0.018           | -0.636 | -4.027 | 0.43           | 0.2  | 4.45   | 4.49   | 1.1            | 0.04            | 0.13            |

| IDN | Zone   | M   | $\sigma_M$ | RA          | Dec        | F275   | F336   | $\sigma_{F275}$ | $\sigma_{F336}$ | x      | y      | $d_n/\sigma_x$ | Age  | log(T) | log(g) | $\sigma_{Age}$ | $\sigma_{logT}$ | $\sigma_{logg}$ |
|-----|--------|-----|------------|-------------|------------|--------|--------|-----------------|-----------------|--------|--------|----------------|------|--------|--------|----------------|-----------------|-----------------|
| 381 | MS     | 9.3 | 1.2        | 152.7272885 | -4.6880533 | 21.578 | 22.116 | 0.022           | 0.02            | -0.611 | -4.436 | -              | 13.7 | 4.44   | 4.29   | 12.6           | 0.03            | 0.13            |
| 382 | MS     | 9.3 | 2.2        | 152.739522  | -4.678972  | 21.649 | 22.189 | 0.039           | 0.019           | -0.613 | -4.365 | -              | 11.8 | 4.44   | 4.32   | 24.9           | 0.05            | 0.23            |
| 383 | MS     | 9.3 | 0.9        | 152.7384917 | -4.6742797 | 21.401 | 21.932 | 0.019           | 0.017           | -0.604 | -4.613 | -              | 18.2 | 4.43   | 4.19   | 8.8            | 0.02            | 0.1             |
| 384 | ZAMS.L | 9.3 | 0.2        | 152.77116   | -4.6965709 | 21.998 | 22.556 | 0.028           | 0.027           | -0.631 | -4.016 | 0.35           | 0.2  | 4.45   | 4.49   | 0.9            | 0.04            | 0.11            |
| 385 | ZAMS.L | 9.3 | 0.3        | 152.7446468 | -4.6776089 | 21.998 | 22.552 | 0.04            | 0.042           | -0.627 | -4.016 | 0.14           | 0.2  | 4.45   | 4.49   | 1.5            | 0.06            | 0.18            |
| 386 | MS     | 9.3 | 1.3        | 152.7560385 | -4.6813715 | 21.482 | 22.016 | 0.024           | 0.028           | -0.607 | -4.532 | -              | 16.6 | 4.43   | 4.23   | 14.5           | 0.04            | 0.17            |
| 387 | TAMS.R | 9.3 | 0.9        | 152.7490754 | -4.6774678 | 20.689 | 21.152 | 0.02            | 0.017           | -0.536 | -5.325 | 0.54           | 28.1 | 4.36   | 3.71   | 7.9            | 0.02            | 0.11            |
| 388 | MS     | 9.3 | 0.7        | 152.7447897 | -4.678537  | 20.843 | 21.33  | 0.023           | 0.021           | -0.56  | -5.171 | -              | 26.8 | 4.38   | 3.81   | 5.7            | 0.03            | 0.11            |
| 389 | ZAMS.L | 9.3 | 0.2        | 152.7299494 | -4.6846225 | 22.01  | 22.601 | 0.025           | 0.022           | -0.664 | -4.004 | 1.73           | 0.2  | 4.45   | 4.49   | 0.8            | 0.03            | 0.1             |
| 390 | MS     | 9.3 | 1.1        | 152.7444624 | -4.671531  | 21.459 | 21.991 | 0.023           | 0.021           | -0.605 | -4.555 | -              | 17.6 | 4.43   | 4.22   | 11.2           | 0.03            | 0.13            |
| 391 | MS     | 9.3 | 1.6        | 152.7339933 | -4.6903809 | 21.46  | 21.992 | 0.034           | 0.028           | -0.605 | -4.554 | -              | 17.6 | 4.43   | 4.22   | 16.5           | 0.04            | 0.19            |
| 392 | MS     | 9.3 | 0.9        | 152.7681051 | -4.6997394 | 21.357 | 21.884 | 0.021           | 0.011           | -0.6   | -4.657 | -              | 19.8 | 4.43   | 4.16   | 8.7            | 0.03            | 0.11            |
| 393 | MS     | 9.3 | 2.7        | 152.7254607 | -4.6890398 | 21.874 | 22.415 | 0.041           | 0.035           | -0.614 | -4.14  | -              | 5.4  | 4.44   | 4.41   | 28.2           | 0.05            | 0.27            |
| 394 | MS     | 9.2 | 1.4        | 152.7286965 | -4.6939471 | 21.492 | 22.025 | 0.031           | 0.025           | -0.606 | -4.522 | -              | 17   | 4.43   | 4.23   | 14.7           | 0.04            | 0.17            |
| 395 | MS     | 9.2 | 0.9        | 152.7624526 | -4.698274  | 21.327 | 21.852 | 0.022           | 0.021           | -0.598 | -4.687 | -              | 20.6 | 4.42   | 4.14   | 8.7            | 0.03            | 0.12            |
| 396 | MS     | 9.2 | 1.1        | 152.7416427 | -4.6790418 | 21.474 | 22.006 | 0.021           | 0.024           | -0.605 | -4.54  | -              | 17.6 | 4.43   | 4.22   | 11.7           | 0.03            | 0.14            |
| 397 | MS     | 9.2 | 0.9        | 152.7210223 | -4.6840435 | 21.189 | 21.705 | 0.025           | 0.018           | -0.589 | -4.825 | -              | 23   | 4.41   | 4.05   | 8.1            | 0.03            | 0.12            |
| 398 | ZAMS.L | 9.2 | 0.3        | 152.7686115 | -4.7058748 | 22.023 | 22.616 | 0.035           | 0.024           | -0.666 | -3.991 | 1.31           | 0.2  | 4.45   | 4.49   | 1.2            | 0.05            | 0.14            |
| 399 | TAMS.R | 9.2 | 1.1        | 152.7256161 | -4.6966974 | 20.711 | 21.182 | 0.024           | 0.022           | -0.544 | -5.303 | 0.09           | 28.5 | 4.36   | 3.71   | 9.7            | 0.03            | 0.13            |
| 400 | MS     | 9.2 | 2.1        | 152.7339019 | -4.6735797 | 21.794 | 22.334 | 0.037           | 0.026           | -0.613 | -4.22  | -              | 8.9  | 4.44   | 4.37   | 24.7           | 0.05            | 0.22            |
| 401 | MS     | 9.2 | 0.6        | 152.767672  | -4.701828  | 21.073 | 21.578 | 0.02            | 0.014           | -0.578 | -4.941 | -              | 25.2 | 4.4    | 3.96   | 5.3            | 0.02            | 0.09            |
| 402 | TAMS.R | 9.2 | 1.1        | 152.7410898 | -4.6694869 | 20.719 | 21.187 | 0.024           | 0.025           | -0.541 | -5.295 | 0.2            | 28.7 | 4.36   | 3.71   | 9.9            | 0.03            | 0.14            |
| 403 | ZAMS.L | 9.2 | 0.2        | 152.7313452 | -4.7149257 | 22.038 | 22.596 | 0.041           | 0.03            | -0.631 | -3.976 | 0.28           | 0.2  | 4.45   | 4.49   | 1.3            | 0.05            | 0.16            |
| 404 | MS     | 9.2 | 2          | 152.7252803 | -4.6902818 | 21.761 | 22.3   | 0.034           | 0.029           | -0.612 | -4.253 | -              | 10.5 | 4.44   | 4.35   | 23.9           | 0.04            | 0.21            |
| 405 | ZAMS.L | 9.2 | 0.2        | 152.7288957 | -4.6843491 | 22.04  | 22.59  | 0.032           | 0.02            | -0.623 | -3.974 | 0.12           | 0.2  | 4.45   | 4.49   | 1              | 0.04            | 0.12            |
| 406 | MS     | 9.2 | 0.7        | 152.7410125 | -4.6765745 | 21.24  | 21.757 | 0.021           | 0.016           | -0.59  | -4.774 | -              | 23   | 4.41   | 4.07   | 6.4            | 0.03            | 0.1             |
| 407 | TAMS.R | 9.1 | 0.9        | 152.7571895 | -4.710674  | 20.732 | 21.173 | 0.019           | 0.018           | -0.514 | -5.282 | 1.65           | 29   | 4.36   | 3.71   | 7.7            | 0.02            | 0.1             |
| 408 | TAMS.R | 9.1 | 1.1        | 152.7234067 | -4.6884636 | 20.73  | 21.17  | 0.025           | 0.025           | -0.513 | -5.284 | 1.3            | 29   | 4.36   | 3.71   | 10.1           | 0.03            | 0.14            |
| 409 | MS     | 9.1 | 1.6        | 152.7654319 | -4.6878597 | 21.694 | 22.231 | 0.032           | 0.025           | -0.61  | -4.32  | -              | 12.9 | 4.44   | 4.32   | 17.3           | 0.04            | 0.18            |
| 410 | MS     | 9.1 | 2.2        | 152.726043  | -4.6980858 | 21.635 | 22.17  | 0.047           | 0.026           | -0.608 | -4.379 | -              | 14.8 | 4.44   | 4.29   | 24             | 0.06            | 0.26            |
| 411 | MS     | 9.1 | 0.8        | 152.7573901 | -4.6778204 | 20.864 | 21.347 | 0.03            | 0.023           | -0.556 | -5.15  | -              | 27.9 | 4.37   | 3.8    | 6.7            | 0.04            | 0.13            |
| 412 | MS     | 9.1 | 1          | 152.7329417 | -4.6909293 | 21.27  | 21.788 | 0.029           | 0.025           | -0.591 | -4.744 | -              | 22.8 | 4.42   | 4.08   | 9.3            | 0.04            | 0.14            |
| 413 | MS     | 9.1 | 1.5        | 152.7411342 | -4.6743738 | 21.676 | 22.212 | 0.028           | 0.031           | -0.609 | -4.338 | -              | 13.7 | 4.44   | 4.31   | 17.7           | 0.04            | 0.19            |
| 414 | MS     | 9.1 | 1          | 152.7242042 | -4.688413  | 21.409 | 21.935 | 0.025           | 0.028           | -0.599 | -4.605 | -              | 20.2 | 4.42   | 4.17   | 10.4           | 0.03            | 0.15            |
| 415 | MS     | 9.1 | 1.6        | 152.7487341 | -4.6780151 | 21.583 | 22.116 | 0.035           | 0.032           | -0.606 | -4.431 | -              | 16.4 | 4.43   | 4.26   | 17.4           | 0.04            | 0.19            |
| 416 | MS     | 9.1 | 1.6        | 152.7565662 | -4.678707  | 21.541 | 22.072 | 0.039           | 0.029           | -0.604 | -4.473 | -              | 17.7 | 4.43   | 4.24   | 17.5           | 0.05            | 0.21            |
| 417 | MS     | 9.1 | 1.4        | 152.7317739 | -4.7151917 | 21.048 | 21.547 | 0.049           | 0.034           | -0.572 | -4.966 | -              | 26.4 | 4.39   | 3.93   | 12.3           | 0.06            | 0.22            |
| 418 | ZAMS.L | 9.1 | 0.2        | 152.7608943 | -4.6960814 | 22.074 | 22.624 | 0.033           | 0.038           | -0.623 | -3.94  | 0.14           | 0.2  | 4.45   | 4.49   | 1.3            | 0.05            | 0.15            |
| 419 | MS     | 9   | 1.7        | 152.7643923 | -4.6980843 | 21.996 | 22.534 | 0.035           | 0.026           | -0.611 | -4.018 | -              | 3.2  | 4.44   | 4.43   | 22.1           | 0.04            | 0.2             |
| 420 | MS     | 9   | 1          | 152.7295064 | -4.6990706 | 22.068 | 22.608 | 0.049           | 0.038           | -0.613 | -3.946 | -              | 0.5  | 4.44   | 4.47   | 7.2            | 0.06            | 0.22            |
| 421 | MS     | 9   | 0.5        | 152.7401138 | -4.6947015 | 20.878 | 21.359 | 0.02            | 0.017           | -0.554 | -5.136 | -              | 28.5 | 4.37   | 3.79   | 4.5            | 0.02            | 0.09            |
| 422 | MS     | 9   | 1          | 152.7279061 | -4.6894013 | 21.056 | 21.554 | 0.032           | 0.037           | -0.571 | -4.958 | -              | 26.7 | 4.39   | 3.92   | 8.9            | 0.05            | 0.18            |
| 423 | MS     | 9   | 1.1        | 152.7375258 | -4.6769412 | 21.417 | 21.941 | 0.028           | 0.023           | -0.597 | -4.597 | -              | 21   | 4.42   | 4.16   | 10.8           | 0.03            | 0.14            |
| 424 | ZAMS.L | 9   | 0.2        | 152.7271509 | -4.6943096 | 22.083 | 22.633 | 0.042           | 0.036           | -0.623 | -3.931 | 0.14           | 0.2  | 4.45   | 4.49   | 1.4            | 0.06            | 0.16            |
| 425 | MS     | 9   | 1.2        | 152.7484446 | -4.6714553 | 21.382 | 21.904 | 0.033           | 0.024           | -0.595 | -4.632 | -              | 21.7 | 4.42   | 4.14   | 12.2           | 0.04            | 0.17            |

| IDN | Zone   | M   | $\sigma_M$ | RA          | Dec        | F275   | F336   | $\sigma_{F275}$ | $\sigma_{F336}$ | x      | y      | $d_n/\sigma_x$ | Age  | log(T) | log(g) | $\sigma_{Age}$ | $\sigma_{logT}$ | $\sigma_{logg}$ |
|-----|--------|-----|------------|-------------|------------|--------|--------|-----------------|-----------------|--------|--------|----------------|------|--------|--------|----------------|-----------------|-----------------|
| 426 | MS     | 9   | 1.1        | 152.719424  | -4.6911267 | 21.282 | 21.797 | 0.024           | 0.036           | -0.588 | -4.732 | -              | 23.8 | 4.41   | 4.07   | 11.1           | 0.04            | 0.19            |
| 427 | TAMS.R | 9   | 0.8        | 152.7706669 | -4.7010752 | 20.77  | 21.219 | 0.018           | 0.018           | -0.522 | -5.244 | 1.22           | 29.9 | 4.36   | 3.72   | 7.3            | 0.02            | 0.1             |
| 428 | MS     | 9   | 0.5        | 152.764958  | -4.7041243 | 21.156 | 21.661 | 0.013           | 0.018           | -0.578 | -4.858 | -              | 25.9 | 4.4    | 3.99   | 4.9            | 0.02            | 0.09            |
| 429 | MS     | 9   | 1          | 152.7377927 | -4.675986  | 20.919 | 21.402 | 0.038           | 0.017           | -0.556 | -5.095 | -              | 28.6 | 4.37   | 3.81   | 8.7            | 0.05            | 0.17            |
| 430 | MS     | 9   | 0.6        | 152.7444883 | -4.6785284 | 21.224 | 21.734 | 0.02            | 0.019           | -0.583 | -4.79  | -              | 25   | 4.41   | 4.03   | 5.9            | 0.02            | 0.1             |
| 431 | ZAMS.L | 9   | 0.3        | 152.7245346 | -4.6861634 | 22.096 | 22.677 | 0.049           | 0.028           | -0.654 | -3.918 | 0.77           | 0.2  | 4.45   | 4.49   | 1.6            | 0.06            | 0.19            |
| 432 | MS     | 9   | 0.2        | 152.7268703 | -4.6908532 | 22.102 | 22.645 | 0.032           | 0.032           | -0.616 | -3.912 | -              | 0.2  | 4.45   | 4.49   | 1.1            | 0.04            | 0.13            |
| 433 | TAMS.R | 9   | 0.9        | 152.7705092 | -4.6983464 | 20.783 | 21.241 | 0.021           | 0.022           | -0.531 | -5.231 | 0.57           | 30.2 | 4.36   | 3.72   | 8.7            | 0.03            | 0.12            |
| 434 | TAMS.R | 9   | 0.8        | 152.7580418 | -4.6900202 | 20.785 | 21.208 | 0.035           | 0.026           | -0.496 | -5.229 | 1.35           | 30.2 | 4.36   | 3.72   | 7.9            | 0.04            | 0.15            |
| 435 | MS     | 9   | 0.5        | 152.7441833 | -4.6926984 | 20.915 | 21.396 | 0.026           | 0.019           | -0.554 | -5.099 | -              | 29   | 4.37   | 3.8    | 4.3            | 0.03            | 0.11            |
| 436 | MS     | 8.9 | 0.9        | 152.7716723 | -4.6989164 | 21.534 | 22.061 | 0.031           | 0.029           | -0.6   | -4.48  | -              | 19.4 | 4.43   | 4.21   | 9.8            | 0.04            | 0.15            |
| 437 | MS     | 8.9 | 1.2        | 152.7389727 | -4.6732566 | 21.834 | 22.37  | 0.021           | 0.028           | -0.609 | -4.18  | -              | 10.8 | 4.44   | 4.36   | 17.1           | 0.04            | 0.16            |
| 438 | MS     | 8.9 | 0.8        | 152.7503772 | -4.6831231 | 20.801 | 21.272 | 0.031           | 0.021           | -0.544 | -5.213 | -              | 30.1 | 4.36   | 3.72   | 7.6            | 0.04            | 0.14            |
| 439 | MS     | 8.9 | 1.2        | 152.7431476 | -4.684548  | 21.698 | 22.231 | 0.036           | 0.034           | -0.606 | -4.316 | -              | 15.1 | 4.43   | 4.3    | 14.6           | 0.04            | 0.18            |
| 440 | MS     | 8.9 | 0.4        | 152.7265238 | -4.6864693 | 21.195 | 21.701 | 0.017           | 0.021           | -0.579 | -4.819 | -              | 25.8 | 4.4    | 4      | 4.2            | 0.03            | 0.1             |
| 441 | MS     | 8.9 | 0.5        | 152.7474456 | -4.668821  | 20.833 | 21.305 | 0.023           | 0.023           | -0.545 | -5.181 | -              | 29.9 | 4.36   | 3.74   | 4.1            | 0.03            | 0.1             |
| 442 | MS     | 8.9 | 1          | 152.73904   | -4.6896373 | 21.643 | 22.174 | 0.03            | 0.027           | -0.604 | -4.371 | -              | 16.8 | 4.43   | 4.27   | 11.7           | 0.04            | 0.15            |
| 443 | MS     | 8.9 | 0.4        | 152.7471045 | -4.6770347 | 20.841 | 21.314 | 0.018           | 0.016           | -0.546 | -5.173 | -              | 29.8 | 4.36   | 3.75   | 3.2            | 0.02            | 0.08            |
| 444 | ZAMS.L | 8.9 | 0.2        | 152.7271765 | -4.6855989 | 22.115 | 22.677 | 0.043           | 0.027           | -0.635 | -3.899 | 0.45           | 0.2  | 4.44   | 4.49   | 1.4            | 0.05            | 0.16            |
| 445 | MS     | 8.9 | 0.7        | 152.72449   | -4.699666  | 20.889 | 21.366 | 0.04            | 0.037           | -0.55  | -5.125 | -              | 29.4 | 4.37   | 3.78   | 6.6            | 0.05            | 0.17            |
| 446 | ZAMS.L | 8.9 | 0.3        | 152.732656  | -4.7073783 | 22.121 | 22.7   | 0.052           | 0.034           | -0.652 | -3.893 | 0.71           | 0.2  | 4.44   | 4.49   | 1.7            | 0.07            | 0.19            |
| 447 | TAMS.R | 8.9 | 0.8        | 152.7425446 | -4.6932886 | 20.799 | 21.236 | 0.033           | 0.023           | -0.51  | -5.215 | 0.99           | 30.4 | 4.36   | 3.72   | 7.5            | 0.04            | 0.14            |
| 448 | ZAMS.L | 8.9 | 0.2        | 152.7429909 | -4.6756943 | 22.122 | 22.69  | 0.036           | 0.039           | -0.641 | -3.892 | 0.66           | 0.2  | 4.44   | 4.49   | 1.3            | 0.05            | 0.15            |
| 449 | TAMS.R | 8.9 | 0.8        | 152.7364565 | -4.7185875 | 20.808 | 21.23  | 0.035           | 0.026           | -0.495 | -5.206 | 1.35           | 30.6 | 4.36   | 3.72   | 7.9            | 0.04            | 0.15            |
| 450 | MS     | 8.9 | 1.5        | 152.7464514 | -4.6965866 | 21.687 | 22.218 | 0.045           | 0.031           | -0.604 | -4.327 | -              | 16.1 | 4.43   | 4.28   | 17.2           | 0.06            | 0.22            |
| 451 | MS     | 8.9 | 0.4        | 152.7465156 | -4.6729243 | 21.224 | 21.73  | 0.02            | 0.022           | -0.579 | -4.79  | -              | 25.9 | 4.4    | 4.01   | 4.6            | 0.03            | 0.1             |
| 452 | MS     | 8.9 | 0.3        | 152.7514956 | -4.6781083 | 20.934 | 21.413 | 0.015           | 0.019           | -0.552 | -5.08  | -              | 29.4 | 4.37   | 3.8    | 3              | 0.02            | 0.08            |
| 453 | MS     | 8.9 | 0.6        | 152.7526427 | -4.6811615 | 21.226 | 21.732 | 0.027           | 0.03            | -0.579 | -4.788 | -              | 25.9 | 4.4    | 4.01   | 6.3            | 0.04            | 0.14            |
| 454 | MS     | 8.9 | 0.4        | 152.7270984 | -4.6884978 | 21.106 | 21.601 | 0.022           | 0.02            | -0.568 | -4.908 | -              | 27.7 | 4.39   | 3.92   | 4              | 0.03            | 0.09            |
| 455 | MS     | 8.9 | 1.5        | 152.742392  | -4.6749476 | 22.028 | 22.563 | 0.028           | 0.021           | -0.608 | -3.986 | -              | 4.3  | 4.44   | 4.43   | 21.3           | 0.04            | 0.17            |
| 456 | MS     | 8.9 | 0.3        | 152.7399371 | -4.6750824 | 20.989 | 21.473 | 0.015           | 0.016           | -0.557 | -5.025 | -              | 29   | 4.37   | 3.84   | 2.6            | 0.02            | 0.07            |
| 457 | MS     | 8.9 | 1          | 152.7272217 | -4.6924791 | 21.645 | 22.174 | 0.033           | 0.021           | -0.602 | -4.369 | -              | 17.5 | 4.43   | 4.26   | 11.8           | 0.04            | 0.16            |
| 458 | MS     | 8.9 | 1.7        | 152.7328978 | -4.7146376 | 22.069 | 22.604 | 0.037           | 0.03            | -0.608 | -3.945 | -              | 2.7  | 4.44   | 4.44   | 22.5           | 0.05            | 0.21            |
| 459 | TAMS.R | 8.9 | 0.5        | 152.744496  | -4.674995  | 20.82  | 21.252 | 0.021           | 0.021           | -0.505 | -5.194 | 1.74           | 30.7 | 4.36   | 3.72   | 4.8            | 0.03            | 0.1             |
| 460 | ZAMS.L | 8.9 | 0.2        | 152.7253009 | -4.6889544 | 22.14  | 22.732 | 0.04            | 0.026           | -0.665 | -3.874 | 1.27           | 0.2  | 4.44   | 4.49   | 1.3            | 0.05            | 0.15            |
| 461 | MS     | 8.9 | 0.6        | 152.76005   | -4.6824726 | 20.97  | 21.451 | 0.034           | 0.026           | -0.554 | -5.044 | -              | 29.3 | 4.37   | 3.82   | 5.6            | 0.04            | 0.14            |
| 462 | MS     | 8.9 | 1          | 152.7560607 | -4.6731624 | 21.73  | 22.261 | 0.029           | 0.022           | -0.604 | -4.284 | -              | 15.4 | 4.43   | 4.3    | 11.8           | 0.04            | 0.15            |
| 463 | MS     | 8.8 | 0.7        | 152.7580716 | -4.7067205 | 21.614 | 22.141 | 0.023           | 0.018           | -0.6   | -4.4   | -              | 18.6 | 4.43   | 4.24   | 7.7            | 0.03            | 0.11            |
| 464 | MS     | 8.8 | 1          | 152.7577951 | -4.6909262 | 21.738 | 22.269 | 0.03            | 0.032           | -0.604 | -4.276 | -              | 15.3 | 4.43   | 4.3    | 13.6           | 0.04            | 0.17            |
| 465 | MS     | 8.8 | 0.5        | 152.751024  | -4.7089369 | 21.251 | 21.756 | 0.023           | 0.022           | -0.578 | -4.763 | -              | 26.1 | 4.4    | 4.01   | 4.9            | 0.03            | 0.1             |
| 466 | ZAMS.L | 8.8 | 0.1        | 152.740416  | -4.6801095 | 22.146 | 22.701 | 0.023           | 0.025           | -0.628 | -3.868 | 0.56           | 0.2  | 4.44   | 4.49   | 0.9            | 0.03            | 0.1             |
| 467 | ZAMS.L | 8.8 | 0.1        | 152.7403191 | -4.675878  | 22.147 | 22.705 | 0.028           | 0.035           | -0.631 | -3.867 | 0.49           | 0.2  | 4.44   | 4.49   | 1.2            | 0.04            | 0.14            |
| 468 | MS     | 8.8 | 0.8        | 152.7638727 | -4.7046274 | 21.633 | 22.16  | 0.025           | 0.019           | -0.6   | -4.381 | -              | 18.4 | 4.43   | 4.24   | 9.4            | 0.03            | 0.12            |
| 469 | ZAMS.L | 8.8 | 0.1        | 152.7702938 | -4.702408  | 22.157 | 22.72  | 0.018           | 0.024           | -0.636 | -3.857 | 0.95           | 0.2  | 4.44   | 4.49   | 0.8            | 0.03            | 0.09            |
| 470 | TAMS.R | 8.8 | 0.5        | 152.7536245 | -4.6989042 | 20.843 | 21.282 | 0.022           | 0.024           | -0.512 | -5.171 | 1.18           | 31.1 | 4.35   | 3.72   | 5.4            | 0.03            | 0.11            |

| IDN | Zone   | M   | $\sigma_M$ | RA          | Dec        | F275   | F336   | $\sigma_{F275}$ | $\sigma_{F336}$ | x      | y      | $d_n/\sigma_x$ | Age  | log(T) | log(g) | $\sigma_{Age}$ | $\sigma_{logT}$ | $\sigma_{logg}$ |
|-----|--------|-----|------------|-------------|------------|--------|--------|-----------------|-----------------|--------|--------|----------------|------|--------|--------|----------------|-----------------|-----------------|
| 471 | MS     | 8.8 | 1.7        | 152.7230853 | -4.6950005 | 22.105 | 22.639 | 0.04            | 0.024           | -0.607 | -3.909 | -              | 2.2  | 4.43   | 4.45   | 24.8           | 0.05            | 0.22            |
| 472 | ZAMS L | 8.8 | 0.1        | 152.7451313 | -4.7068965 | 22.16  | 22.732 | 0.026           | 0.034           | -0.645 | -3.854 | 0.94           | 0.2  | 4.44   | 4.49   | 1.2            | 0.04            | 0.13            |
| 473 | ZAMS L | 8.8 | 0.2        | 152.7398101 | -4.7207303 | 22.164 | 22.721 | 0.044           | 0.023           | -0.63  | -3.85  | 0.39           | 0.2  | 4.44   | 4.49   | 1.4            | 0.06            | 0.16            |
| 474 | MS     | 8.8 | 0.9        | 152.7271478 | -4.7016435 | 21.392 | 21.905 | 0.039           | 0.028           | -0.586 | -4.622 | -              | 24.2 | 4.41   | 4.1    | 9.7            | 0.05            | 0.18            |
| 475 | MS     | 8.8 | 0.9        | 152.7540601 | -4.6983186 | 21.435 | 21.95  | 0.037           | 0.029           | -0.588 | -4.579 | -              | 23.6 | 4.41   | 4.12   | 9.5            | 0.04            | 0.17            |
| 476 | MS     | 8.8 | 0.6        | 152.7421101 | -4.6806628 | 21.087 | 21.574 | 0.029           | 0.025           | -0.56  | -4.927 | -              | 29   | 4.38   | 3.88   | 5.2            | 0.04            | 0.12            |
| 477 | MS     | 8.8 | 1.1        | 152.7238485 | -4.6930549 | 21.646 | 22.171 | 0.039           | 0.027           | -0.598 | -4.368 | -              | 19   | 4.42   | 4.24   | 13.6           | 0.05            | 0.19            |
| 478 | TAMS R | 8.8 | 0.5        | 152.7372507 | -4.6728737 | 20.865 | 21.303 | 0.019           | 0.022           | -0.511 | -5.149 | 1.27           | 31.4 | 4.35   | 3.72   | 4.9            | 0.03            | 0.1             |
| 479 | MS     | 8.8 | 0.5        | 152.7712965 | -4.7020603 | 22.173 | 22.709 | 0.029           | 0.031           | -0.609 | -3.841 | -              | 0.3  | 4.44   | 4.48   | 4.5            | 0.04            | 0.14            |
| 480 | MS     | 8.7 | 0.4        | 152.7643902 | -4.7037703 | 21.308 | 21.813 | 0.014           | 0.018           | -0.578 | -4.706 | -              | 26.2 | 4.4    | 4.03   | 4              | 0.02            | 0.09            |
| 481 | TAMS R | 8.7 | 0.7        | 152.7456376 | -4.6815094 | 20.869 | 21.314 | 0.03            | 0.018           | -0.518 | -5.145 | 0.69           | 31.4 | 4.35   | 3.72   | 6.8            | 0.04            | 0.13            |
| 482 | MS     | 8.7 | 0.7        | 152.7592305 | -4.6921681 | 21.526 | 22.045 | 0.027           | 0.026           | -0.592 | -4.488 | -              | 22   | 4.42   | 4.17   | 8              | 0.03            | 0.13            |
| 483 | TAMS R | 8.7 | 0.7        | 152.7621056 | -4.6944378 | 20.869 | 21.287 | 0.031           | 0.033           | -0.491 | -5.145 | 1.45           | 31.4 | 4.35   | 3.72   | 7.4            | 0.04            | 0.16            |
| 484 | ZAMS L | 8.7 | 0.1        | 152.7281367 | -4.6817946 | 22.182 | 22.74  | 0.024           | 0.029           | -0.631 | -3.832 | 0.66           | 0.2  | 4.44   | 4.49   | 1              | 0.04            | 0.11            |
| 485 | ZAMS L | 8.7 | 0.2        | 152.7243618 | -4.6885919 | 22.184 | 22.783 | 0.044           | 0.035           | -0.672 | -3.83  | 1.37           | 0.2  | 4.44   | 4.49   | 1.4            | 0.06            | 0.16            |
| 486 | MS     | 8.7 | 0.8        | 152.7247177 | -4.6941742 | 21.391 | 21.901 | 0.034           | 0.024           | -0.583 | -4.623 | -              | 25   | 4.41   | 4.08   | 8.1            | 0.04            | 0.15            |
| 487 | ZAMS L | 8.7 | 0.3        | 152.732153  | -4.7052794 | 22.193 | 22.786 | 0.05            | 0.037           | -0.666 | -3.821 | 1.09           | 0.2  | 4.44   | 4.49   | 1.7            | 0.06            | 0.18            |
| 488 | MS     | 8.7 | 0.4        | 152.7506616 | -4.6782175 | 20.995 | 21.469 | 0.021           | 0.018           | -0.547 | -5.019 | -              | 30.6 | 4.36   | 3.8    | 3.5            | 0.03            | 0.09            |
| 489 | MS     | 8.7 | 0.5        | 152.7508969 | -4.6742942 | 21.237 | 21.734 | 0.024           | 0.022           | -0.57  | -4.777 | -              | 27.7 | 4.39   | 3.97   | 4.9            | 0.03            | 0.1             |
| 490 | MS     | 8.7 | 1          | 152.7392092 | -4.6994926 | 21.634 | 22.156 | 0.035           | 0.027           | -0.595 | -4.38  | -              | 20.2 | 4.42   | 4.22   | 11.4           | 0.04            | 0.17            |
| 491 | MS     | 8.7 | 0.6        | 152.7465525 | -4.6785506 | 21.198 | 21.691 | 0.026           | 0.034           | -0.566 | -4.816 | -              | 28.4 | 4.39   | 3.94   | 6.4            | 0.04            | 0.15            |
| 492 | MS     | 8.7 | 0.6        | 152.7312456 | -4.6831212 | 21.517 | 22.033 | 0.02            | 0.025           | -0.589 | -4.497 | -              | 22.9 | 4.41   | 4.15   | 7.1            | 0.03            | 0.12            |
| 493 | MS     | 8.7 | 0.5        | 152.7275051 | -4.6996936 | 21.08  | 21.561 | 0.025           | 0.022           | -0.554 | -4.934 | -              | 30   | 4.37   | 3.85   | 4.3            | 0.03            | 0.1             |
| 494 | TAMS R | 8.7 | 0.7        | 152.7462433 | -4.6995831 | 20.897 | 21.325 | 0.028           | 0.02            | -0.501 | -5.117 | 1.29           | 31.9 | 4.35   | 3.72   | 6.9            | 0.03            | 0.12            |
| 495 | ZAMS L | 8.7 | 0.2        | 152.7474815 | -4.6770791 | 22.202 | 22.746 | 0.037           | 0.028           | -0.617 | -3.812 | 0.16           | 0.2  | 4.44   | 4.49   | 1.2            | 0.05            | 0.13            |
| 496 | MS     | 8.7 | 2          | 152.7444074 | -4.709573  | 22.109 | 22.64  | 0.028           | 0.038           | -0.604 | -3.905 | -              | 4.2  | 4.43   | 4.43   | 31.5           | 0.05            | 0.24            |
| 497 | MS     | 8.7 | 2.2        | 152.7539603 | -4.6954325 | 22.086 | 22.617 | 0.042           | 0.019           | -0.604 | -3.928 | -              | 5.2  | 4.43   | 4.42   | 31.8           | 0.05            | 0.25            |
| 498 | MS     | 8.7 | 0.5        | 152.7312599 | -4.6854653 | 20.934 | 21.4   | 0.025           | 0.019           | -0.539 | -5.08  | -              | 31.6 | 4.35   | 3.74   | 4.5            | 0.03            | 0.1             |
| 499 | TAMS R | 8.7 | 0.5        | 152.7254382 | -4.6866711 | 20.901 | 21.355 | 0.02            | 0.022           | -0.527 | -5.113 | 0.45           | 31.9 | 4.35   | 3.72   | 5.4            | 0.03            | 0.1             |
| 500 | MS     | 8.7 | 0.5        | 152.7269951 | -4.7001435 | 21.226 | 21.72  | 0.026           | 0.024           | -0.567 | -4.788 | -              | 28.3 | 4.39   | 3.96   | 5.1            | 0.03            | 0.11            |
| 501 | TAMS R | 8.6 | 0.7        | 152.7444947 | -4.676476  | 20.907 | 21.341 | 0.028           | 0.021           | -0.507 | -5.107 | 1.06           | 32   | 4.35   | 3.72   | 6.9            | 0.03            | 0.12            |
| 502 | MS     | 8.6 | 1.1        | 152.7252811 | -4.6830014 | 21.701 | 22.224 | 0.036           | 0.023           | -0.596 | -4.313 | -              | 19.1 | 4.42   | 4.25   | 13.4           | 0.04            | 0.17            |
| 503 | ZAMS L | 8.6 | 0.3        | 152.7404052 | -4.691698  | 22.217 | 22.825 | 0.056           | 0.043           | -0.681 | -3.797 | 1.27           | 0.2  | 4.44   | 4.5    | 1.9            | 0.07            | 0.2             |
| 504 | MS     | 8.6 | 0.5        | 152.7635861 | -4.7007888 | 21.251 | 21.746 | 0.026           | 0.022           | -0.568 | -4.763 | -              | 28.2 | 4.39   | 3.97   | 5.1            | 0.03            | 0.11            |
| 505 | ZAMS L | 8.6 | 0.2        | 152.7648131 | -4.7026098 | 22.221 | 22.774 | 0.033           | 0.02            | -0.626 | -3.793 | 0.49           | 0.2  | 4.44   | 4.5    | 1.1            | 0.04            | 0.12            |
| 506 | TAMS R | 8.6 | 0.8        | 152.7512664 | -4.6940044 | 20.914 | 21.321 | 0.032           | 0.022           | -0.48  | -5.1   | 1.76           | 32.2 | 4.35   | 3.72   | 7.9            | 0.04            | 0.14            |
| 507 | TAMS R | 8.6 | 0.5        | 152.7715232 | -4.6995353 | 20.915 | 21.349 | 0.019           | 0.018           | -0.507 | -5.099 | 1.53           | 32.2 | 4.35   | 3.72   | 4.7            | 0.02            | 0.09            |
| 508 | TAMS R | 8.6 | 0.8        | 152.7556717 | -4.6778145 | 20.913 | 21.349 | 0.03            | 0.018           | -0.509 | -5.101 | 0.91           | 32.1 | 4.35   | 3.72   | 7.4            | 0.03            | 0.13            |
| 509 | MS     | 8.6 | 0.9        | 152.7483227 | -4.6674948 | 21.492 | 22.004 | 0.031           | 0.04            | -0.585 | -4.522 | -              | 24.2 | 4.41   | 4.12   | 11             | 0.05            | 0.19            |
| 510 | MS     | 8.6 | 1.5        | 152.7428031 | -4.6767243 | 21.993 | 22.523 | 0.037           | 0.034           | -0.603 | -4.021 | -              | 9.9  | 4.43   | 4.38   | 21.5           | 0.05            | 0.2             |
| 511 | MS     | 8.6 | 1.2        | 152.7205559 | -4.6900552 | 21.725 | 22.248 | 0.041           | 0.023           | -0.596 | -4.289 | -              | 18.8 | 4.42   | 4.25   | 15.2           | 0.05            | 0.2             |
| 512 | MS     | 8.6 | 1          | 152.746628  | -4.6721635 | 21.781 | 22.306 | 0.033           | 0.019           | -0.598 | -4.233 | -              | 17.1 | 4.42   | 4.28   | 12.9           | 0.04            | 0.16            |
| 513 | MS     | 8.6 | 0.9        | 152.7468606 | -4.6731215 | 21.488 | 21.999 | 0.036           | 0.02            | -0.584 | -4.526 | -              | 24.4 | 4.41   | 4.12   | 9.2            | 0.04            | 0.16            |
| 514 | MS     | 8.6 | 0.9        | 152.7548349 | -4.6737616 | 21.664 | 22.184 | 0.031           | 0.029           | -0.593 | -4.35  | -              | 20.6 | 4.42   | 4.22   | 10.1           | 0.04            | 0.15            |
| 515 | MS     | 8.6 | 1.1        | 152.7517187 | -4.702209  | 21.779 | 22.303 | 0.034           | 0.029           | -0.597 | -4.235 | -              | 17.6 | 4.42   | 4.28   | 13.3           | 0.04            | 0.17            |

| IDN | Zone   | M   | $\sigma_M$ | RA          | Dec        | F275   | F336   | $\sigma_{F275}$ | $\sigma_{F336}$ | x      | y      | $d_n/\sigma_x$ | Age  | log(T) | log(g) | $\sigma_{Age}$ | $\sigma_{logT}$ | $\sigma_{logg}$ |
|-----|--------|-----|------------|-------------|------------|--------|--------|-----------------|-----------------|--------|--------|----------------|------|--------|--------|----------------|-----------------|-----------------|
| 516 | MS     | 8.6 | 0.8        | 152.7304176 | -4.6853488 | 21.699 | 22.22  | 0.028           | 0.029           | -0.594 | -4.315 | -              | 19.8 | 4.42   | 4.23   | 10.3           | 0.04            | 0.15            |
| 517 | TAMS R | 8.6 | 0.6        | 152.7718178 | -4.7031714 | 20.929 | 21.386 | 0.022           | 0.019           | -0.53  | -5.085 | 0.24           | 32.4 | 4.35   | 3.72   | 5.5            | 0.03            | 0.1             |
| 518 | MS     | 8.6 | 1.1        | 152.7546333 | -4.689462  | 21.576 | 22.091 | 0.044           | 0.035           | -0.588 | -4.438 | -              | 22.9 | 4.41   | 4.16   | 12.9           | 0.05            | 0.2             |
| 519 | MS     | 8.6 | 0.9        | 152.7307857 | -4.681656  | 21.722 | 22.244 | 0.031           | 0.021           | -0.595 | -4.292 | -              | 19.2 | 4.42   | 4.25   | 11.5           | 0.04            | 0.15            |
| 520 | MS     | 8.6 | 0.4        | 152.7438203 | -4.6748671 | 21.045 | 21.517 | 0.021           | 0.021           | -0.545 | -4.969 | -              | 31.2 | 4.36   | 3.8    | 3.5            | 0.03            | 0.09            |
| 521 | ZAMS L | 8.6 | 0.2        | 152.7664952 | -4.706985  | 22.236 | 22.866 | 0.032           | 0.052           | -0.703 | -3.778 | 1.81           | 0.2  | 4.44   | 4.5    | 1.8            | 0.06            | 0.2             |
| 522 | MS     | 8.6 | 2.4        | 152.7644051 | -4.7080761 | 22.068 | 22.597 | 0.05            | 0.04            | -0.602 | -3.946 | -              | 7.7  | 4.43   | 4.4    | 32.4           | 0.06            | 0.29            |
| 523 | MS     | 8.6 | 1.1        | 152.7695305 | -4.7046035 | 22.156 | 22.685 | 0.022           | 0.018           | -0.602 | -3.858 | -              | 3.7  | 4.43   | 4.44   | 19             | 0.03            | 0.13            |
| 524 | MS     | 8.6 | 0.6        | 152.7389147 | -4.7123327 | 21.431 | 21.936 | 0.028           | 0.026           | -0.578 | -4.583 | -              | 26.1 | 4.4    | 4.07   | 6.9            | 0.03            | 0.13            |
| 525 | MS     | 8.6 | 0.4        | 152.7424626 | -4.7087331 | 21.265 | 21.757 | 0.021           | 0.018           | -0.565 | -4.749 | -              | 28.8 | 4.38   | 3.96   | 4.2            | 0.03            | 0.09            |
| 526 | TAMS R | 8.6 | 0.6        | 152.7424522 | -4.7037146 | 20.942 | 21.393 | 0.024           | 0.024           | -0.524 | -5.072 | 0.44           | 32.6 | 4.35   | 3.72   | 6              | 0.03            | 0.11            |
| 527 | TAMS R | 8.5 | 0.4        | 152.766479  | -4.6942391 | 20.946 | 21.37  | 0.017           | 0.019           | -0.497 | -5.068 | 1.96           | 32.7 | 4.35   | 3.73   | 4.7            | 0.02            | 0.09            |
| 528 | MS     | 8.5 | 1.4        | 152.7520034 | -4.6744407 | 21.985 | 22.513 | 0.036           | 0.025           | -0.601 | -4.029 | -              | 11.4 | 4.43   | 4.37   | 21.2           | 0.04            | 0.19            |
| 529 | MS     | 8.5 | 0.7        | 152.7279497 | -4.6858598 | 21.712 | 22.232 | 0.024           | 0.021           | -0.593 | -4.302 | -              | 20   | 4.42   | 4.23   | 8.7            | 0.03            | 0.11            |
| 530 | MS     | 8.5 | 0.6        | 152.7540127 | -4.7110303 | 21.643 | 22.16  | 0.021           | 0.022           | -0.59  | -4.371 | -              | 21.8 | 4.41   | 4.2    | 7.2            | 0.03            | 0.11            |
| 531 | MS     | 8.5 | 0.7        | 152.7274043 | -4.6926532 | 22.227 | 22.757 | 0.043           | 0.037           | -0.603 | -3.787 | -              | 0.8  | 4.43   | 4.47   | 5.8            | 0.05            | 0.18            |
| 532 | MS     | 8.5 | 0.5        | 152.7420547 | -4.669822  | 21.228 | 21.716 | 0.025           | 0.026           | -0.561 | -4.786 | -              | 29.4 | 4.38   | 3.93   | 4.8            | 0.03            | 0.12            |
| 533 | MS     | 8.5 | 0.5        | 152.7368471 | -4.7098861 | 21.192 | 21.676 | 0.025           | 0.02            | -0.557 | -4.822 | -              | 30   | 4.37   | 3.9    | 4.5            | 0.03            | 0.1             |
| 534 | MS     | 8.5 | 1          | 152.7241881 | -4.6993832 | 21.806 | 22.329 | 0.033           | 0.033           | -0.596 | -4.208 | -              | 17.6 | 4.42   | 4.28   | 14             | 0.04            | 0.17            |
| 535 | MS     | 8.5 | 0.9        | 152.726098  | -4.6956353 | 21.46  | 21.966 | 0.041           | 0.019           | -0.579 | -4.554 | -              | 25.8 | 4.4    | 4.08   | 10.1           | 0.05            | 0.18            |
| 536 | MS     | 8.5 | 0.6        | 152.7275265 | -4.7029209 | 21.409 | 21.911 | 0.027           | 0.023           | -0.575 | -4.605 | -              | 26.9 | 4.4    | 4.05   | 6.5            | 0.03            | 0.12            |
| 537 | MS     | 8.5 | 0.5        | 152.7257676 | -4.6886244 | 21.158 | 21.638 | 0.029           | 0.019           | -0.553 | -4.856 | -              | 30.5 | 4.37   | 3.87   | 5.1            | 0.03            | 0.12            |
| 538 | MS     | 8.5 | 0.4        | 152.7407083 | -4.6710585 | 21.246 | 21.734 | 0.02            | 0.021           | -0.561 | -4.768 | -              | 29.5 | 4.38   | 3.93   | 3.9            | 0.03            | 0.09            |
| 539 | MS     | 8.5 | 0.9        | 152.7604369 | -4.7065558 | 21.9   | 22.425 | 0.028           | 0.022           | -0.598 | -4.114 | -              | 15   | 4.42   | 4.32   | 13.1           | 0.03            | 0.14            |
| 540 | MS     | 8.5 | 2.7        | 152.7391701 | -4.6932622 | 22.168 | 22.696 | 0.052           | 0.042           | -0.601 | -3.846 | -              | 4.1  | 4.43   | 4.44   | 32.7           | 0.06            | 0.31            |
| 541 | MS     | 8.5 | 0.9        | 152.7645175 | -4.688588  | 21.696 | 22.213 | 0.03            | 0.036           | -0.59  | -4.318 | -              | 21.3 | 4.41   | 4.21   | 12.6           | 0.04            | 0.18            |
| 542 | MS     | 8.5 | 0.5        | 152.7339133 | -4.6857195 | 21.022 | 21.485 | 0.024           | 0.019           | -0.536 | -4.992 | -              | 32.6 | 4.35   | 3.76   | 4.4            | 0.03            | 0.1             |
| 543 | MS     | 8.5 | 0.7        | 152.7460456 | -4.7087262 | 21.275 | 21.763 | 0.038           | 0.028           | -0.561 | -4.739 | -              | 29.6 | 4.38   | 3.94   | 7.4            | 0.05            | 0.16            |
| 544 | MS     | 8.5 | 0.7        | 152.7400932 | -4.7082198 | 21.333 | 21.826 | 0.034           | 0.028           | -0.566 | -4.681 | -              | 28.8 | 4.39   | 3.98   | 7              | 0.04            | 0.14            |
| 545 | TAMS R | 8.5 | 0.9        | 152.7484295 | -4.6840881 | 20.971 | 21.397 | 0.035           | 0.032           | -0.499 | -5.043 | 0.96           | 33.1 | 4.35   | 3.73   | 8.7            | 0.04            | 0.15            |
| 546 | MS     | 8.5 | 0.9        | 152.7681597 | -4.705787  | 21.403 | 21.902 | 0.026           | 0.045           | -0.572 | -4.611 | -              | 27.6 | 4.39   | 4.03   | 10.4           | 0.05            | 0.21            |
| 547 | MS     | 8.5 | 1.1        | 152.7345367 | -4.7010182 | 21.713 | 22.23  | 0.04            | 0.031           | -0.59  | -4.301 | -              | 21.1 | 4.41   | 4.22   | 13.4           | 0.05            | 0.19            |
| 548 | MS     | 8.5 | 0.9        | 152.7403604 | -4.7200084 | 21.64  | 22.153 | 0.034           | 0.028           | -0.586 | -4.374 | -              | 23.1 | 4.41   | 4.18   | 10.1           | 0.04            | 0.16            |
| 549 | TAMS R | 8.4 | 0.6        | 152.7228617 | -4.6879478 | 20.98  | 21.419 | 0.024           | 0.018           | -0.512 | -5.034 | 0.84           | 33.3 | 4.35   | 3.73   | 6.2            | 0.03            | 0.11            |
| 550 | ZAMS L | 8.4 | 0.2        | 152.7309747 | -4.6860438 | 22.282 | 22.819 | 0.032           | 0.036           | -0.61  | -3.732 | 0.09           | 0.2  | 4.43   | 4.5    | 1.3            | 0.04            | 0.14            |
| 551 | MS     | 8.4 | 0.4        | 152.7290166 | -4.6868179 | 21.288 | 21.775 | 0.022           | 0.021           | -0.56  | -4.726 | -              | 29.8 | 4.38   | 3.94   | 4.3            | 0.03            | 0.09            |
| 552 | MS     | 8.4 | 2          | 152.7510846 | -4.6816615 | 22.04  | 22.566 | 0.049           | 0.048           | -0.599 | -3.974 | -              | 11   | 4.42   | 4.38   | 29.3           | 0.06            | 0.27            |
| 553 | MS     | 8.4 | 0.7        | 152.7278225 | -4.6854065 | 21.446 | 21.946 | 0.029           | 0.019           | -0.573 | -4.568 | -              | 27.3 | 4.39   | 4.05   | 6.9            | 0.04            | 0.13            |
| 554 | MS     | 8.4 | 0.7        | 152.7485965 | -4.6798076 | 21.394 | 21.889 | 0.033           | 0.022           | -0.568 | -4.62  | -              | 28.4 | 4.39   | 4.01   | 7.3            | 0.04            | 0.14            |
| 555 | MS     | 8.4 | 1.1        | 152.7271271 | -4.7000767 | 21.629 | 22.14  | 0.042           | 0.031           | -0.584 | -4.385 | -              | 23.8 | 4.41   | 4.16   | 12             | 0.05            | 0.19            |
| 556 | MS     | 8.4 | 0.7        | 152.7285658 | -4.6765781 | 21.319 | 21.808 | 0.033           | 0.03            | -0.562 | -4.695 | -              | 29.5 | 4.38   | 3.96   | 6.6            | 0.04            | 0.14            |
| 557 | TAMS R | 8.4 | 0.4        | 152.7596542 | -4.7083144 | 20.998 | 21.446 | 0.015           | 0.017           | -0.521 | -5.016 | 0.59           | 33.6 | 4.34   | 3.73   | 4.4            | 0.02            | 0.08            |
| 558 | ZAMS L | 8.4 | 0.2        | 152.763889  | -4.7061482 | 22.299 | 22.856 | 0.036           | 0.023           | -0.63  | -3.715 | 0.67           | 0.2  | 4.43   | 4.5    | 1.2            | 0.04            | 0.13            |
| 559 | MS     | 8.4 | 0.5        | 152.7328771 | -4.7086852 | 21.167 | 21.64  | 0.03            | 0.018           | -0.546 | -4.847 | -              | 31.8 | 4.36   | 3.84   | 5.1            | 0.04            | 0.12            |
| 560 | MS     | 8.4 | 1          | 152.7543876 | -4.6766598 | 21.771 | 22.288 | 0.034           | 0.022           | -0.59  | -4.243 | -              | 20.4 | 4.41   | 4.24   | 12             | 0.04            | 0.16            |
| 561 | MS     | 8.4 | 0.7        | 152.7404676 | -4.6856726 | 21.444 | 21.942 | 0.034           | 0.028           | -0.571 | -4.57  | -              | 27.8 | 4.39   | 4.04   | 7.8            | 0.04            | 0.15            |
| 562 | MS     | 8.4 | 0.6        | 152.7205493 | -4.6976479 | 21.059 | 21.521 | 0.032           | 0.023           | -0.535 | -4.955 | -              | 32.9 | 4.35   | 3.76   | 5.8            | 0.04            | 0.13            |

| IDN | Zone   | M   | $\sigma_M$ | RA          | Dec        | F275   | F336   | $\sigma_{F275}$ | $\sigma_{F336}$ | x      | y      | $d_n/\sigma_x$ | Age  | log(T) | log(g) | $\sigma_{Age}$ | $\sigma_{logT}$ | $\sigma_{logg}$ |
|-----|--------|-----|------------|-------------|------------|--------|--------|-----------------|-----------------|--------|--------|----------------|------|--------|--------|----------------|-----------------|-----------------|
| 563 | TAMS.R | 8.4 | 0.6        | 152.7537092 | -4.6953124 | 21.008 | 21.429 | 0.024           | 0.02            | -0.494 | -5.006 | 1.52           | 33.7 | 4.34   | 3.73   | 6.2            | 0.03            | 0.11            |
| 564 | MS     | 8.4 | 0.7        | 152.743762  | -4.6803332 | 21.572 | 22.078 | 0.026           | 0.03            | -0.579 | -4.442 | -              | 25.5 | 4.4    | 4.12   | 8              | 0.04            | 0.15            |
| 565 | ZAMS.L | 8.4 | 0.2        | 152.7388897 | -4.6750582 | 22.305 | 22.881 | 0.032           | 0.026           | -0.649 | -3.709 | 1.36           | 0.2  | 4.43   | 4.5    | 1.1            | 0.04            | 0.11            |
| 566 | MS     | 8.4 | 0.8        | 152.7402521 | -4.6819306 | 21.635 | 22.144 | 0.03            | 0.02            | -0.582 | -4.379 | -              | 24.3 | 4.4    | 4.15   | 8.7            | 0.04            | 0.14            |
| 567 | MS     | 8.4 | 0.6        | 152.7704518 | -4.6949945 | 21.495 | 21.995 | 0.02            | 0.027           | -0.573 | -4.519 | -              | 27.3 | 4.39   | 4.07   | 6.4            | 0.03            | 0.13            |
| 568 | ZAMS.L | 8.3 | 0.2        | 152.7738924 | -4.7007675 | 22.317 | 22.888 | 0.03            | 0.03            | -0.644 | -3.697 | 1.31           | 0.2  | 4.43   | 4.5    | 1.1            | 0.04            | 0.11            |
| 569 | MS     | 8.3 | 0.2        | 152.7568484 | -4.6945148 | 22.315 | 22.845 | 0.031           | 0.035           | -0.603 | -3.699 | -              | 0.3  | 4.43   | 4.49   | 1.2            | 0.04            | 0.13            |
| 570 | ZAMS.L | 8.3 | 0.3        | 152.7463615 | -4.682104  | 22.317 | 22.854 | 0.056           | 0.041           | -0.61  | -3.697 | 0.09           | 0.2  | 4.43   | 4.5    | 1.9            | 0.07            | 0.2             |
| 571 | ZAMS.L | 8.3 | 0.2        | 152.7543923 | -4.6694107 | 22.318 | 22.866 | 0.045           | 0.033           | -0.621 | -3.696 | 0.36           | 0.2  | 4.43   | 4.5    | 1.5            | 0.06            | 0.16            |
| 572 | MS     | 8.3 | 0.6        | 152.7429375 | -4.6811973 | 21.374 | 21.864 | 0.031           | 0.027           | -0.563 | -4.64  | -              | 29.5 | 4.38   | 3.98   | 6.4            | 0.04            | 0.13            |
| 573 | MS     | 8.3 | 1          | 152.7581392 | -4.7091835 | 21.907 | 22.427 | 0.025           | 0.031           | -0.593 | -4.107 | -              | 17.2 | 4.42   | 4.3    | 14             | 0.04            | 0.16            |
| 574 | ZAMS.L | 8.3 | 0.2        | 152.7475611 | -4.7101475 | 22.327 | 22.865 | 0.036           | 0.033           | -0.611 | -3.687 | 0.19           | 0.2  | 4.43   | 4.5    | 1.2            | 0.04            | 0.13            |
| 575 | ZAMS.L | 8.3 | 0.2        | 152.7494286 | -4.6727489 | 22.328 | 22.889 | 0.04            | 0.047           | -0.634 | -3.686 | 0.64           | 0.2  | 4.43   | 4.5    | 1.7            | 0.06            | 0.18            |
| 576 | MS     | 8.3 | 0.5        | 152.7298254 | -4.6880193 | 21.41  | 21.901 | 0.019           | 0.019           | -0.564 | -4.604 | -              | 29.3 | 4.38   | 4      | 5.8            | 0.03            | 0.12            |
| 577 | MS     | 8.3 | 0.5        | 152.740867  | -4.6794433 | 21.501 | 21.999 | 0.023           | 0.015           | -0.571 | -4.513 | -              | 27.7 | 4.39   | 4.06   | 5.6            | 0.03            | 0.1             |
| 578 | MS     | 8.3 | 0.5        | 152.7595836 | -4.7050991 | 21.462 | 21.957 | 0.022           | 0.025           | -0.568 | -4.552 | -              | 28.5 | 4.39   | 4.03   | 5.9            | 0.03            | 0.12            |
| 579 | MS     | 8.3 | 0.8        | 152.7378157 | -4.699272  | 21.695 | 22.205 | 0.031           | 0.02            | -0.583 | -4.319 | -              | 23.6 | 4.41   | 4.18   | 9.6            | 0.04            | 0.14            |
| 580 | MS     | 8.3 | 0.3        | 152.7445926 | -4.6853682 | 21.23  | 21.704 | 0.019           | 0.021           | -0.547 | -4.784 | -              | 31.9 | 4.36   | 3.87   | 3.5            | 0.02            | 0.09            |
| 581 | MS     | 8.3 | 1.4        | 152.7472137 | -4.6706136 | 22.261 | 22.785 | 0.035           | 0.032           | -0.597 | -3.753 | -              | 3.3  | 4.42   | 4.45   | 22.1           | 0.04            | 0.18            |
| 582 | MS     | 8.3 | 0.5        | 152.7404023 | -4.67651   | 21.311 | 21.792 | 0.027           | 0.022           | -0.554 | -4.703 | -              | 31   | 4.37   | 3.92   | 5.2            | 0.03            | 0.11            |
| 583 | ZAMS.L | 8.3 | 0.3        | 152.7269183 | -4.6875712 | 22.339 | 22.916 | 0.047           | 0.031           | -0.65  | -3.675 | 0.99           | 0.2  | 4.43   | 4.5    | 1.6            | 0.06            | 0.17            |
| 584 | TAMS.R | 8.3 | 1          | 152.7547504 | -4.6912019 | 21.046 | 21.471 | 0.04            | 0.02            | -0.498 | -4.968 | 0.75           | 34.4 | 4.34   | 3.73   | 10.3           | 0.05            | 0.18            |
| 585 | MS     | 8.3 | 0.4        | 152.7332984 | -4.6979723 | 21.092 | 21.55  | 0.018           | 0.023           | -0.531 | -4.922 | -              | 33.8 | 4.34   | 3.76   | 4.1            | 0.03            | 0.1             |
| 586 | TAMS.R | 8.3 | 1          | 152.7305274 | -4.6954168 | 21.045 | 21.451 | 0.039           | 0.031           | -0.479 | -4.969 | 1.26           | 34.4 | 4.34   | 3.73   | 10.1           | 0.04            | 0.17            |
| 587 | MS     | 8.3 | 1.1        | 152.7290609 | -4.688389  | 21.885 | 22.402 | 0.037           | 0.035           | -0.59  | -4.129 | -              | 18.8 | 4.41   | 4.28   | 15.5           | 0.04            | 0.18            |
| 588 | TAMS.R | 8.3 | 1.2        | 152.7419589 | -4.6793136 | 21.046 | 21.459 | 0.049           | 0.022           | -0.486 | -4.968 | 0.86           | 34.4 | 4.34   | 3.73   | 12.7           | 0.06            | 0.22            |
| 589 | MS     | 8.3 | 0.6        | 152.7373063 | -4.7210126 | 21.225 | 21.696 | 0.031           | 0.028           | -0.544 | -4.789 | -              | 32.4 | 4.36   | 3.85   | 5.4            | 0.04            | 0.13            |
| 590 | TAMS.R | 8.3 | 0.7        | 152.7573326 | -4.6794924 | 21.048 | 21.468 | 0.028           | 0.029           | -0.493 | -4.966 | 1.2            | 34.4 | 4.34   | 3.73   | 7.5            | 0.03            | 0.14            |
| 591 | ZAMS.L | 8.3 | 0.3        | 152.7507184 | -4.6820832 | 22.347 | 22.92  | 0.05            | 0.026           | -0.646 | -3.667 | 0.86           | 0.2  | 4.43   | 4.5    | 1.7            | 0.06            | 0.18            |
| 592 | MS     | 8.3 | 1.9        | 152.7269725 | -4.6966602 | 22.172 | 22.695 | 0.034           | 0.04            | -0.596 | -3.842 | -              | 8.3  | 4.42   | 4.41   | 33.4           | 0.05            | 0.24            |
| 593 | MS     | 8.2 | 0.7        | 152.7691457 | -4.6966636 | 21.516 | 22.012 | 0.03            | 0.023           | -0.569 | -4.498 | -              | 28.2 | 4.39   | 4.05   | 7.3            | 0.04            | 0.13            |
| 594 | TAMS.R | 8.2 | 0.8        | 152.7618956 | -4.6954046 | 21.057 | 21.456 | 0.033           | 0.022           | -0.472 | -4.957 | 1.68           | 34.6 | 4.34   | 3.73   | 8.5            | 0.04            | 0.15            |
| 595 | MS     | 8.2 | 2.7        | 152.7223413 | -4.6980632 | 22.227 | 22.75  | 0.054           | 0.03            | -0.596 | -3.787 | -              | 5.8  | 4.42   | 4.43   | 34.3           | 0.07            | 0.31            |
| 596 | MS     | 8.2 | 1.2        | 152.7626227 | -4.7034893 | 22.017 | 22.537 | 0.037           | 0.029           | -0.593 | -3.997 | -              | 14.9 | 4.42   | 4.34   | 17.4           | 0.04            | 0.18            |
| 597 | MS     | 8.2 | 0.6        | 152.7461536 | -4.6859828 | 21.201 | 21.668 | 0.033           | 0.033           | -0.54  | -4.813 | -              | 32.9 | 4.35   | 3.83   | 5.6            | 0.04            | 0.14            |
| 598 | MS     | 8.2 | 0.7        | 152.7281484 | -4.6888328 | 22.345 | 22.87  | 0.036           | 0.047           | -0.598 | -3.669 | -              | 0.6  | 4.42   | 4.48   | 6.7            | 0.06            | 0.21            |
| 599 | MS     | 8.2 | 1.2        | 152.7665533 | -4.7012681 | 22.126 | 22.648 | 0.032           | 0.031           | -0.595 | -3.888 | -              | 10.9 | 4.42   | 4.38   | 18.9           | 0.04            | 0.17            |
| 600 | MS     | 8.2 | 1.1        | 152.7254035 | -4.6865713 | 21.718 | 22.226 | 0.043           | 0.035           | -0.581 | -4.296 | -              | 24.1 | 4.4    | 4.18   | 13.4           | 0.05            | 0.2             |
| 601 | ZAMS.L | 8.2 | 0.2        | 152.7279489 | -4.6854181 | 22.362 | 22.956 | 0.039           | 0.034           | -0.667 | -3.652 | 1.66           | 0.2  | 4.43   | 4.5    | 1.3            | 0.05            | 0.14            |
| 602 | MS     | 8.2 | 1.7        | 152.7337546 | -4.6978976 | 22.322 | 22.845 | 0.042           | 0.029           | -0.596 | -3.692 | -              | 1.8  | 4.42   | 4.46   | 25.9           | 0.05            | 0.22            |
| 603 | MS     | 8.2 | 0.7        | 152.7438814 | -4.6791732 | 21.535 | 22.031 | 0.034           | 0.021           | -0.569 | -4.479 | -              | 28.2 | 4.39   | 4.06   | 8.2            | 0.04            | 0.15            |
| 604 | ZAMS.L | 8.2 | 0.2        | 152.7427927 | -4.6762469 | 22.365 | 22.919 | 0.044           | 0.034           | -0.627 | -3.649 | 0.57           | 0.2  | 4.43   | 4.5    | 1.5            | 0.05            | 0.16            |
| 605 | MS     | 8.2 | 1.3        | 152.7296333 | -4.6756632 | 21.951 | 22.468 | 0.041           | 0.031           | -0.59  | -4.063 | -              | 17.7 | 4.41   | 4.3    | 18.3           | 0.05            | 0.2             |
| 606 | ZAMS.L | 8.2 | 0.3        | 152.7526083 | -4.681675  | 22.364 | 22.945 | 0.051           | 0.047           | -0.654 | -3.65  | 1.02           | 0.2  | 4.43   | 4.5    | 1.8            | 0.06            | 0.18            |
| 607 | ZAMS.L | 8.2 | 0.2        | 152.7511457 | -4.674458  | 22.368 | 22.978 | 0.044           | 0.035           | -0.683 | -3.646 | 1.84           | 0.2  | 4.43   | 4.5    | 1.5            | 0.05            | 0.16            |
| 608 | MS     | 8.2 | 1          | 152.7294267 | -4.6834261 | 22.024 | 22.543 | 0.031           | 0.031           | -0.592 | -3.99  | -              | 15.3 | 4.42   | 4.33   | 15.2           | 0.04            | 0.16            |

| IDN | Zone   | M   | $\sigma_M$ | RA          | Dec        | F275   | F336   | $\sigma_{F275}$ | $\sigma_{F336}$ | x      | y      | $d_n/\sigma_x$ | Age  | log(T) | log(g) | $\sigma_{Age}$ | $\sigma_{logT}$ | $\sigma_{logg}$ |
|-----|--------|-----|------------|-------------|------------|--------|--------|-----------------|-----------------|--------|--------|----------------|------|--------|--------|----------------|-----------------|-----------------|
| 609 | TAMS.R | 8.2 | 0.9        | 152.7352183 | -4.6973116 | 21.077 | 21.495 | 0.043           | 0.034           | -0.491 | -4.937 | 0.82           | 34.9 | 4.34   | 3.73   | 9.4            | 0.05            | 0.18            |
| 610 | MS     | 8.2 | 0.6        | 152.7424416 | -4.7169893 | 21.49  | 21.981 | 0.029           | 0.024           | -0.564 | -4.524 | -              | 29.4 | 4.38   | 4.02   | 6.6            | 0.03            | 0.13            |
| 611 | MS     | 8.2 | 0.7        | 152.7264511 | -4.6880879 | 21.848 | 22.36  | 0.025           | 0.023           | -0.585 | -4.166 | -              | 21.4 | 4.41   | 4.24   | 9.3            | 0.03            | 0.12            |
| 612 | ZAMS.L | 8.2 | 0.2        | 152.7609733 | -4.7001172 | 22.378 | 22.912 | 0.036           | 0.029           | -0.607 | -3.636 | 0.16           | 0.2  | 4.43   | 4.5    | 1.3            | 0.04            | 0.13            |
| 613 | MS     | 8.2 | 0.8        | 152.7265748 | -4.6874002 | 21.902 | 22.416 | 0.027           | 0.026           | -0.587 | -4.112 | -              | 19.8 | 4.41   | 4.27   | 10.5           | 0.03            | 0.13            |
| 614 | MS     | 8.2 | 1.3        | 152.7273396 | -4.7016652 | 21.991 | 22.508 | 0.04            | 0.038           | -0.59  | -4.023 | -              | 16.9 | 4.41   | 4.31   | 17.5           | 0.05            | 0.2             |
| 615 | ZAMS.L | 8.2 | 0.3        | 152.7291562 | -4.6951426 | 22.379 | 22.909 | 0.046           | 0.037           | -0.603 | -3.635 | 0.04           | 0.2  | 4.43   | 4.5    | 1.6            | 0.06            | 0.16            |
| 616 | MS     | 8.2 | 0.9        | 152.7278221 | -4.6857535 | 21.716 | 22.221 | 0.035           | 0.027           | -0.578 | -4.298 | -              | 25   | 4.4    | 4.16   | 10.3           | 0.04            | 0.16            |
| 617 | MS     | 8.1 | 0.6        | 152.7669107 | -4.7051128 | 21.781 | 22.289 | 0.022           | 0.019           | -0.581 | -4.233 | -              | 23.5 | 4.4    | 4.2    | 7.3            | 0.03            | 0.1             |
| 618 | ZAMS.L | 8.1 | 0.3        | 152.743373  | -4.7002849 | 22.389 | 22.957 | 0.049           | 0.035           | -0.641 | -3.625 | 0.82           | 0.2  | 4.43   | 4.5    | 1.7            | 0.06            | 0.17            |
| 619 | MS     | 8.1 | 0.5        | 152.7625583 | -4.7064929 | 21.103 | 21.555 | 0.021           | 0.017           | -0.525 | -4.911 | -              | 35.2 | 4.34   | 3.73   | 5.1            | 0.02            | 0.09            |
| 620 | MS     | 8.1 | 0.9        | 152.7403178 | -4.6761405 | 21.877 | 22.388 | 0.032           | 0.026           | -0.584 | -4.137 | -              | 21.4 | 4.41   | 4.24   | 11.7           | 0.04            | 0.15            |
| 621 | TAMS.R | 8.1 | 0.4        | 152.7687176 | -4.7046604 | 21.11  | 21.557 | 0.018           | 0.016           | -0.52  | -4.904 | 0.23           | 35.3 | 4.34   | 3.73   | 4              | 0.02            | 0.07            |
| 622 | ZAMS.L | 8.1 | 0.2        | 152.7452182 | -4.681286  | 22.396 | 22.931 | 0.037           | 0.04            | -0.608 | -3.618 | 0.19           | 0.2  | 4.43   | 4.5    | 1.5            | 0.05            | 0.15            |
| 623 | MS     | 8.1 | 1.3        | 152.7472559 | -4.6758793 | 21.96  | 22.474 | 0.042           | 0.025           | -0.587 | -4.054 | -              | 18.9 | 4.41   | 4.28   | 17.3           | 0.05            | 0.2             |
| 624 | MS     | 8.1 | 1.7        | 152.75312   | -4.6696229 | 22.359 | 22.88  | 0.044           | 0.045           | -0.594 | -3.655 | -              | 1.8  | 4.42   | 4.46   | 29.3           | 0.05            | 0.25            |
| 625 | MS     | 8.1 | 0.5        | 152.7266797 | -4.6922526 | 21.435 | 21.917 | 0.027           | 0.022           | -0.555 | -4.579 | -              | 31.2 | 4.37   | 3.97   | 5.5            | 0.03            | 0.11            |
| 626 | ZAMS.L | 8.1 | 0.2        | 152.7304635 | -4.6757789 | 22.402 | 22.95  | 0.04            | 0.031           | -0.621 | -3.612 | 0.52           | 0.2  | 4.43   | 4.5    | 1.4            | 0.05            | 0.14            |
| 627 | MS     | 8.1 | 0.6        | 152.7265217 | -4.6910933 | 21.579 | 22.072 | 0.027           | 0.022           | -0.566 | -4.435 | -              | 28.9 | 4.39   | 4.06   | 6.7            | 0.03            | 0.12            |
| 628 | TAMS.R | 8.1 | 0.5        | 152.7489533 | -4.6770882 | 21.121 | 21.564 | 0.024           | 0.018           | -0.516 | -4.893 | 0.32           | 35.5 | 4.34   | 3.73   | 5.3            | 0.03            | 0.1             |
| 629 | MS     | 8.1 | 0.8        | 152.7189583 | -4.6924453 | 21.977 | 22.491 | 0.027           | 0.027           | -0.587 | -4.037 | -              | 18.6 | 4.41   | 4.29   | 11.9           | 0.03            | 0.14            |
| 630 | MS     | 8.1 | 0.7        | 152.7694349 | -4.7054356 | 21.617 | 22.112 | 0.03            | 0.028           | -0.568 | -4.397 | -              | 28.3 | 4.39   | 4.08   | 7.8            | 0.04            | 0.13            |
| 631 | MS     | 8.1 | 1.2        | 152.7418386 | -4.7055863 | 22.057 | 22.573 | 0.038           | 0.038           | -0.589 | -3.957 | -              | 16   | 4.41   | 4.33   | 19.6           | 0.05            | 0.2             |
| 632 | ZAMS.L | 8.1 | 0.2        | 152.7370056 | -4.6749005 | 22.41  | 22.948 | 0.036           | 0.026           | -0.611 | -3.604 | 0.32           | 0.2  | 4.42   | 4.5    | 1.3            | 0.04            | 0.13            |
| 633 | MS     | 8.1 | 0.9        | 152.7616089 | -4.7032399 | 21.921 | 22.432 | 0.026           | 0.033           | -0.584 | -4.093 | -              | 20.8 | 4.41   | 4.26   | 13.9           | 0.04            | 0.17            |
| 634 | MS     | 8.1 | 1          | 152.751196  | -4.696652  | 21.954 | 22.466 | 0.031           | 0.035           | -0.585 | -4.06  | -              | 19.9 | 4.41   | 4.27   | 14.5           | 0.04            | 0.18            |
| 635 | TAMS.R | 8.1 | 0.5        | 152.7343925 | -4.6974973 | 21.132 | 21.549 | 0.025           | 0.02            | -0.49  | -4.882 | 1.32           | 35.7 | 4.34   | 3.73   | 5.5            | 0.03            | 0.1             |
| 636 | MS     | 8.1 | 1.1        | 152.753282  | -4.6748766 | 21.982 | 22.495 | 0.038           | 0.022           | -0.586 | -4.032 | -              | 18.9 | 4.41   | 4.29   | 16.1           | 0.05            | 0.18            |
| 637 | ZAMS.L | 8   | 0.2        | 152.7720059 | -4.7035762 | 22.42  | 22.952 | 0.028           | 0.022           | -0.605 | -3.594 | 0.21           | 0.2  | 4.42   | 4.5    | 1              | 0.03            | 0.1             |
| 638 | MS     | 8   | 0.3        | 152.7653806 | -4.7047061 | 21.258 | 21.719 | 0.019           | 0.018           | -0.534 | -4.756 | -              | 34.2 | 4.35   | 3.82   | 3.2            | 0.02            | 0.08            |
| 639 | TAMS.R | 8   | 0.7        | 152.754428  | -4.6722649 | 21.138 | 21.585 | 0.033           | 0.025           | -0.52  | -4.876 | 0.08           | 35.7 | 4.33   | 3.73   | 7.2            | 0.04            | 0.14            |
| 640 | MS     | 8   | 1          | 152.7238691 | -4.6865806 | 21.909 | 22.419 | 0.034           | 0.032           | -0.583 | -4.105 | -              | 21.3 | 4.41   | 4.25   | 12.8           | 0.04            | 0.16            |
| 641 | MS     | 8   | 0.7        | 152.7691536 | -4.7056398 | 21.714 | 22.214 | 0.029           | 0.026           | -0.573 | -4.3   | -              | 26.5 | 4.39   | 4.14   | 8.5            | 0.04            | 0.13            |
| 642 | MS     | 8   | 1.1        | 152.7265635 | -4.7087422 | 21.96  | 22.472 | 0.036           | 0.031           | -0.585 | -4.054 | -              | 19.8 | 4.41   | 4.27   | 15.6           | 0.04            | 0.17            |
| 643 | MS     | 8   | 0.7        | 152.7446484 | -4.6735078 | 21.464 | 21.945 | 0.035           | 0.02            | -0.554 | -4.55  | -              | 31.5 | 4.37   | 3.97   | 7.2            | 0.04            | 0.15            |
| 644 | MS     | 8   | 0.9        | 152.7313423 | -4.688996  | 21.944 | 22.455 | 0.025           | 0.033           | -0.584 | -4.07  | -              | 20.4 | 4.41   | 4.26   | 13.7           | 0.04            | 0.17            |
| 645 | MS     | 8   | 0.4        | 152.7409181 | -4.7136592 | 21.33  | 21.797 | 0.023           | 0.021           | -0.54  | -4.684 | -              | 33.6 | 4.35   | 3.87   | 4.1            | 0.03            | 0.09            |
| 646 | TAMS.R | 8   | 0.6        | 152.7593468 | -4.7009691 | 21.146 | 21.569 | 0.017           | 0.029           | -0.496 | -4.868 | 0.9            | 35.9 | 4.33   | 3.73   | 6.3            | 0.03            | 0.13            |
| 647 | MS     | 8   | 0.9        | 152.7494201 | -4.6981548 | 21.858 | 22.365 | 0.03            | 0.035           | -0.58  | -4.156 | -              | 23.1 | 4.4    | 4.22   | 13             | 0.04            | 0.17            |
| 648 | MS     | 8   | 0.4        | 152.7317369 | -4.7057078 | 21.256 | 21.715 | 0.023           | 0.021           | -0.532 | -4.758 | -              | 34.6 | 4.35   | 3.81   | 3.9            | 0.03            | 0.09            |
| 649 | ZAMS.L | 8   | 0.3        | 152.7406612 | -4.7076556 | 22.433 | 22.989 | 0.046           | 0.034           | -0.629 | -3.581 | 0.67           | 0.2  | 4.42   | 4.5    | 1.6            | 0.06            | 0.16            |
| 650 | MS     | 8   | 1          | 152.7684107 | -4.7043987 | 21.941 | 22.451 | 0.033           | 0.021           | -0.583 | -4.073 | -              | 20.9 | 4.41   | 4.26   | 13.4           | 0.04            | 0.16            |
| 651 | MS     | 8   | 0.7        | 152.7721412 | -4.6992479 | 21.893 | 22.401 | 0.024           | 0.014           | -0.581 | -4.121 | -              | 22.3 | 4.4    | 4.23   | 9.2            | 0.03            | 0.11            |
| 652 | MS     | 8   | 0.8        | 152.7481702 | -4.6834163 | 21.645 | 22.139 | 0.035           | 0.031           | -0.567 | -4.369 | -              | 28.5 | 4.39   | 4.09   | 9.1            | 0.04            | 0.15            |
| 653 | MS     | 8   | 1.1        | 152.7270131 | -4.6873503 | 22.168 | 22.685 | 0.032           | 0.022           | -0.59  | -3.846 | -              | 12.7 | 4.41   | 4.37   | 18.5           | 0.04            | 0.16            |
| 654 | MS     | 8   | 0.5        | 152.7362118 | -4.6899966 | 21.245 | 21.702 | 0.028           | 0.022           | -0.53  | -4.769 | -              | 34.8 | 4.34   | 3.8    | 4.7            | 0.03            | 0.11            |
| 655 | MS     | 8   | 1.3        | 152.7230417 | -4.6878984 | 22.392 | 22.911 | 0.034           | 0.03            | -0.592 | -3.622 | -              | 1.9  | 4.42   | 4.46   | 21.4           | 0.04            | 0.17            |
